# Supplementary material for: Intrinsic Self-Supervision for Data Quality Audits
Source: arXiv:2305.17048 source file (2024-10-28)
Supplement: Supplementary file 2 [file rebuttal.tex]

\documentclass{article}
\usepackage{graphicx} % Required for inserting images
\usepackage{csquotes}
\usepackage{todonotes}
\usepackage{amssymb} % For the set of real numbers R
\usepackage{amsmath} % For using \text in math mode
\usepackage{url}            % simple URL typesetting
\usepackage[normalem]{ulem}

\usepackage{booktabs}
\usepackage{caption}
\usepackage{subcaption}

\usepackage{multirow}
\usepackage{multicol}

\usepackage{rotating} % for sideways figures and tables
\usepackage{longtable} % for long tables
\usepackage{siunitx}
\sisetup{
    detect-weight=true,
    detect-inline-weight=math,
    separate-uncertainty=true,
}

% Comments
\newcommand{\fabian}[1]{\todo[inline,color=green!20!white]{\textbf{Fabian} #1}}
\newcommand{\simone}[1]{\todo[inline,color=purple!20!white]{\textbf{Simone} #1}}
\newcommand{\alvaro}[1]{\todo[inline,color=blue!20!white]{\textbf{Alvaro} #1}}
\newcommand{\ludovic}[1]{\todo[inline,color=orange!20!white]{\textbf{Ludovic} #1}}
\newcommand{\philippe}[1]{\todo[inline,color=cyan!20!white]{\textbf{Philippe} #1}}
\newcommand{\matt}[1]{\todo[inline,color=cyan!20!white]{\textbf{Matt} #1}}


\title{NeurIPS - SelfClean Rebuttal}
\author{Submission Number: 343}
\date{August 2024}

\begin{document}
% gets rid of the need for the ".\ " at the end
\frenchspacing

\maketitle

% --------------------------------
\section{1st Comments (15 Aug 24)}

\subsection{Review tscY}

\begin{displayquote}
    \textit{R.tscY.1}: In section 5, the identified label errors with SelfClean are compared with human annotators. I would be interesting to report the same for the other benchmarked methods.
\end{displayquote}

We agree that evaluating the rankings produced by other methodologies with human verification, as we did for SelfClean, would provide a more complete picture.
We are setting up this experiment and will post updates on whether it is feasible during the rebuttal period. 

\noindent\rule{8cm}{0.4pt}
\begin{displayquote}
    \textit{R.tscY.2}: The method is compared to prior work. However, the other works are introduced in the appendix not in the main paper.
\end{displayquote}

Due to space constraints and the number of prior works we compare to, we had to introduce them in appendix F rather than the main paper.
This appendix is referenced both at line 182 and in the caption of table 1.

% ----------------------
\newpage
\subsection{Review qYrV}

\subsubsection{Cons}
\begin{displayquote}
    \textit{R.qYrV.1}: Scalability Concerns: While the method is effective, the current formulation may not scale well with extremely large datasets without approximation methods.
\end{displayquote}

We agree that the current formulation does not scale well for near duplicates, as mentioned in appendix B "Limitations".
However, we used multiple engineering tricks, such as memory mapping, multi-threading, and custom implementations, to ensure the current implementation is sufficiently fast for many real use cases.
Please also consult our answer to R.qYrV.5 for specific details on the computational cost of running SelfClean.
We are also testing ideas to improve scaling for very large datasets, such as approximation methods and iterative analysis of nearest-neighbor distances, as mentioned in appendix B "Limitations".

\noindent\rule{8cm}{0.4pt}
\begin{displayquote}
    \textit{R.qYrV.2}: Dependence on Hyperparameters: The automatic cleaning procedure relies on hyperparameters like the contamination rate guess and significance level, which may require careful tuning.
\end{displayquote}

We agree that the automatic cleaning option features some weak dependence on these two hyperparameters as investigated in appendices L.3 and L.4.
Specifically, in L.3 we show that the fraction of found problems does not depend much on the contamination rate guess over several orders of magnitude, and in L.4 that the significance level has a relation that is less than linear with the found problems.

Please note that competing approaches also use similar hyperparameters, such as a contamination rate to set a hard threshold [1].
Furthermore, as described in section 6 "Recommended use" we encourage using SelfClean with a human-in-the-loop that does not feature any additional hyperparameters.

%\ludovic{I would argue that hyperparameters (and their careful tuning) are unavoidable in this use-case. Can you further emphasize that your ranking approach actually use less hyperparameters than competing approaches? Or that they are more intuitive?}
%\philippe{I would agree with Ludovic. I don't necessarily like out "Please note that competing approaches also use similar hyperparameters, such as a contamination rate to set a hard threshold [1]." without an additional information about the why I would prefer an answer similar to what has been done in R.qYrV.6 )}

\noindent\rule{8cm}{0.4pt}
\begin{displayquote}
    \textit{R.qYrV.3}: Comparisons to SOTA: Authors may be encouraged to compare their method to more methods, e.g., Jia et al 2023, Pleiss et al 2020 etc for off-topic samples.
\end{displayquote}

Thank you for suggesting additional methods for comparison. 
We will explore the feasibility of incorporating these during the rebuttal period and will provide updates accordingly. 
However, we would like to clarify that the methods referenced, specifically Jia et al. (2023) and Pleiss et al. (2020), focus on detecting label errors rather than off-topic samples.

\noindent\rule{8cm}{0.4pt}
\begin{displayquote}
    \textit{R.qYrV.4}: Tables Presentation: Figures are well illustrated that readers can know the core methodology very quickly. However, the tables are less easy to understand. For example,
\end{displayquote}

We are aware that some of our tables expose the complexity of evaluating multiple methods on several tasks and datasets.
Unfortunately, the reviewer's comment stops after "[...] For example,".
It would be very useful to have concrete suggestions on how to improve the readability of our tables.

\subsubsection{Opportunities For Improvement}
\begin{displayquote}
    \textit{R.qYrV.5}: Computational Resources: The requirement for self-supervised pre-training on the entire dataset may demand substantial computational resources, which could be a limitation for researchers or practitioners with limited access to high-performance computing.
\end{displayquote}

The computational requirements of the self-supervised pre-training indeed change with the size of the dataset.
For example, the examples provided in the anonymized SelfClean repository can all be run reasonably quickly on Google Colab with GPU acceleration. 
Specifically, for a dataset of 13,000 samples (such as ImageNette) applying SelfClean takes under 1.5 hours with the current implementation on Colab.
For larger datasets pre-training will require more time and computational power.
However, it only has to be carried out once, and model weights can be reused as a starting point for downstream tasks.

\noindent\rule{8cm}{0.4pt}
\begin{displayquote}
    \textit{R.qYrV.6}: Dataset Bias: SELFCLEAN may inherit biases present in the dataset, particularly if the dataset is not diverse or representative of the broader population it aims to serve.
\end{displayquote}

SelfClean may indeed inherit biases present in the dataset, as discussed in appendix B "Limitations".
This was further investigated for off-topic sample detection in the experiment of section H.3, where the results show that, at least in these situations, no systematic bias against underrepresented groups is present.

It is important to note that inherent dataset bias may similarly affect other methodologies requiring the training of a supervised classifier, such as the popular approach of confident learning [3].

\noindent\rule{8cm}{0.4pt}
\begin{displayquote}
    \textit{R.qYrV.7}: Lack of Remediation Strategies: The paper focuses on identifying data quality issues but does not provide extensive strategies for how to remediate these issues once identified.
\end{displayquote}

The paper indeed only focuses on identifying data quality issues as discussed in appendix B "Limitations".
It is our opinion that the tasks of identification and remedy are best discussed separately, as their core can be used independently of each other.
Furthermore, remedial strategies are often specific to the case at hand.
% Note that other works [2], have already built on the proposed methodology and outlined strategies for treating different data quality issues.

\noindent\rule{8cm}{0.4pt}
\begin{displayquote}
    \textit{R.qYrV.8}: Potential Over-Cleaning: There is a risk that the cleaning process might remove valuable outliers or rare cases that, while not fitting the general distribution, are still informative for certain tasks.
\end{displayquote}

The problem of over-cleaning is indeed a reason why the best treatment of data quality issues depends on the specific case.
The focus of the paper is detecting data quality issues and not the improvement of classifier scores.
Furthermore, by resorting to human confirmation (preferably carried out by experts of the respective data subject), we argue that valuable outliers should get treated accordingly.
Please also consult our answer to R.fiv4.1 for more details and a clarification added to the paper.

\noindent\rule{8cm}{0.4pt}
\begin{displayquote}
    \textit{R.qYrV.9}: Human-in-the-loop Trade-offs: Relying on human validation introduces additional complexity and may not be feasible at scale, and there is a risk of introducing human bias into the cleaning process.
\end{displayquote}

% Refer to your own published work in the third person. That is, use “In the previous work of Jones et al. [2]”, not “In our previous work [2]”.
% From: https://neurips.cc/Conferences/2013/PaperInformation/AuthorSubmissionInstructions

We agree that relying on human confirmation requires additional resources.
On the other hand, [2] has already proposed a solution to reduce the effort required for confirmation.

Introducing human bias is indeed a possible result of manual data quality verification.
The process should therefore be performed with due care.
Multiple annotations, cleaning protocols and transparent documentations are some of the measures which can help to mitigate human bias.

\noindent\rule{8cm}{0.4pt}
\begin{displayquote}
    \textit{R.qYrV.10}: Evaluation Methodology: The evaluation of data cleaning frameworks lacks a standard protocol, which may affect the comparability and generalizability of the results.
\end{displayquote}

We agree that the lack of evaluation standards for data cleaning hinders comparisons.
However, we make our evaluation workflow fully available and we encourage practitioners to reuse it.
Furthermore, we release SelfClean's implementation to facilitate its inclusion in future standard benchmarks.
%Together this ensures that even as currently there is no standard, our efforts can be reused. 

\noindent\rule{8cm}{0.4pt}
\begin{displayquote}
    \textit{R.qYrV.11}: Assumption of Data Distribution: The methodology assumes a certain distribution of data quality issues, which may not hold true for all datasets, particularly those with unique characteristics or non-standard contamination.
\end{displayquote}

We agree that there are assumptions about the distribution of data quality issues that influence the effectiveness of the automatic cleaning strategy.
This is one of the reasons why the human-in-the-loop setting is recommended, as violations of the assumptions can be effectively detected.
The fully automatic mode is intended as a means of quickly checking the number of quality issues and estimating the impact of cleaning.

\noindent\rule{8cm}{0.4pt}
\begin{displayquote}
    \textit{R.qYrV.12}: Generalization to Other Types of Data: The SELFCLEAN method has been demonstrated on image datasets; its effectiveness on other types of data, such as text or time-series, is not discussed.
\end{displayquote}

This paper intentionally focuses on identifying data quality issues in image datasets, as discussed in appendix B "Limitations".

\noindent\rule{8cm}{0.4pt}
\begin{displayquote}
    \textit{R.qYrV.13}: Label Granularity: The paper notes that label error detection becomes more challenging as label granularity increases, suggesting that the method may not be as effective for fine-grained classification tasks.
\end{displayquote}

Label error detection may indeed become more difficult as granularity increases as stated in the paper and observed by the reviewer.
However, as summarized in section 5.3 and evaluated in appendix G.3, SelfClean performance stays on par with other benchmarked methods in these settings.

\subsubsection{References}
[1] Zhao, Y., Nasrullah, Z., \& Li, Z. (2019). PyOD: A Python Toolbox for Scalable Outlier Detection.
\\ \noindent
[2] Gröger, F., Lionetti, S., Gottfrois, P., Groh, M., Daneshjou, R., Consortium, L., Navarini, A. A., \& Pouly, M. (2023). Towards Reliable Dermatology Evaluation Benchmarks.
\\ \noindent
[3] Northcutt, C. G., Jiang, L., \& Chuang, I. L. (2021). Confident Learning: Estimating Uncertainty in Dataset Labels.

% ----------------------
\newpage
\subsection{Review fiv4}

\subsubsection{Major Weaknesses}

\begin{displayquote}
    \textit{R.fiv4.1}: The authors define samples as off-topic when they are included in the dataset by mistake and consider them outliers in the feature space. However, the hidden stratification [1] phenomenon is not well-considered in this case. For example, when some subsets of the samples have low prevalence (e.g., 100 white dog images and one black dog image), the black dog image has a high potential to be determined as an outlier. Therefore, simply using ‘mistakes' to represent off-topic samples is not rigorous. It would be better to discuss more about this phenomenon in the main paper and Section H.3.
\end{displayquote}

We completely agree with the reviewer that the \emph{candidate} off-topic samples detected by SelfClean are not necessarily mistakes, as discussed in general for candidate data quality issues at the start of "Recommended use" in section 6.
However, we rather see the off-topic ranking as a useful tool to expose hidden stratification, as it highlights which samples are considered to be global or local outliers by a model that is trained without labels.
Moreover, the potential negative effects of off-topic sample cleaning in the presence of hidden stratification are indirectly explored in appendix H.3, where we use metadata to examine bias against minority groups which are not known during model training.

We appreciate the reviewer's comment, as it highlights that the discussion of off-topic samples should be improved to immediately clarify that, although we are looking for mistakes, it may detect atypical but correct samples.
The following clarification will be included in our revision at line 131 between "some examples." and "We achieve":
"Atypical samples, due e.g.\ to the phenomenon of hidden stratification [1], may be included intentionally, and although they are not off-topic they may be revealed in the same search, but require different treatment."

%\matt{Can you be more direct and concise here? We define off-topic samples as "..." where ... shows a precise definition that clarifies that off-topic is different than a label error or a "mistake." I know right now, we define it as "\textit{Off-topic samples}, i.e., inputs included in a dataset by mistake, add noise to evaluation metrics while slowing down and confusing training." Perhaps, we could slightly change the definition: \textit{Off-topic samples}, i.e., inputs included in a dataset unintentionally which add noise to evaluation metrics while slowing down and confusing training. "Unintentionally" helps clarify that there's an intention that must exist and off-topic is related to the intention of the dataset or task creator. Also, can we include an example sentence directly in the paper where we write: Imagine 100 images of Lyme disease in light skin and then one image of Lyme disease in dark skin and another image of a radiology scan, SelfClean may rank the dark skin image as different than the 100 light skin images but the radiology scan will be ranked as way more different. This is a draft sentence, and I think this helps the reader build intuition and avoid making the mistake the reviewer did here. }

\noindent\rule{8cm}{0.4pt}
\begin{displayquote}
    \textit{R.fiv4.2}: The effect of near duplicate samples on model performance is unclear. For example, if removing duplicate samples does not affect model evaluation, the importance of this issue will be lower than other types.
\end{displayquote}

The most prominent effect of near duplicates is when they cause a train-evaluation leakage and thus produce overly optimistic performance estimates.
This can be seen in Table 3 for Fitzpatrick17k where cleaning the evaluation set and data leaks results in significantly lower performance (-4.1\%pt. in F1).
As shown in Table 16, this dataset contains 15\% of near duplicates, but only a very small number of off-topic samples and label errors, so the effect can be attributed to lifting data leaks.
In our experience, important data leaks are a common pattern since training-evaluation splits are often performed randomly, thus causing near-duplicate samples to be assigned to different splits and significantly changing performance scores through memorization.

On the other hand, near duplicate pairs within the same data split may re-weight samples in an uncontrolled way, which may affect score estimates for evaluation splits and learning dynamics for the training split.
Their influence in this setting is more limited for the datasets we considered so far, but we argue that information on near duplicates is anyways valuable and allows to handle all of these scenarios correctly.
This point is now briefly included in a second paragraph of section 6 "Influence of dataset cleaning", which can be found in the answer to R.fiv4.4.

\noindent\rule{8cm}{0.4pt}
\begin{displayquote}
    \textit{R.fiv4.3}: [2] defines four types of label errors. It would be better to show more analysis. The current version seems to only consider correctable label errors (label flip issue).
\end{displayquote}

We thank the reviewer for pointing this out and agree that a more detailed analysis on the type of label error is interesting.
Following the suggestion, we computed the alignment of the SelfClean label error ranking for each of the four types of label errors using a reannotated version of ImageNet-1k [2].
Results show that label error rankings correspond best to correctable errors, and worst to samples with low annotator agreement.
Across all four types SelfClean outperforms competitors by a clear margin.

\begin{table}[htbp]
    \centering
    % \caption{
    %     Comparison of \textsc{SelfClean} and competitor rankings with metadata from multiple benchmark datasets.
    %     We include the proportion of positive samples, which corresponds to the baseline AP.
    % }
    \resizebox{1.0\linewidth}{!}{%
    \begin{tabular}{l c ll rr}
        \toprule
        \bfseries Label Error Type & 
        \bfseries $\text{Positive Samples (\%)}$ & 
        \bfseries Method &
        \bfseries Rep. &
        \bfseries $\text{AUROC (\%)}$ & 
        \bfseries $\text{AP (\%)}$ \\
        
        \midrule
        \multirow{3}{*}{Correctable} & \multirow{3}{*}{2.9} 
            & CLearning & INet & 44.4 & 2.9 \\
        & 
            & FastDup & INet & 60.0 & 3.8 \\
        & 
            & \textsc{SelfClean} & DINO & \textbf{66.2} & \textbf{5.4} \\
        \midrule
        \multirow{3}{*}{Multi-label} & \multirow{3}{*}{1.2} 
            & CLearning & INet & 55.1 & 1.3 \\
        & 
            & FastDup & INet & 63.4 & 1.8 \\
        & 
            & \textsc{SelfClean} & DINO & \textbf{67.7} & \textbf{2.6} \\
        \midrule
        \multirow{3}{*}{Neither} & \multirow{3}{*}{0.6} 
            & CLearning & INet & 52.2 & 0.6 \\
        & 
            & FastDup & INet & 65.8 & 0.8 \\
        & 
            & \textsc{SelfClean} & DINO & \textbf{69.5} & \textbf{1.2} \\
        \midrule
        \multirow{3}{*}{Non-agreement} & \multirow{3}{*}{1.2} 
            & CLearning & INet & 50.5 & 1.3 \\
        & 
            & FastDup & INet & 62.0 & 1.7 \\
        & 
            & \textsc{SelfClean} & DINO & \textbf{65.3} & \textbf{1.9} \\
        \bottomrule
    \end{tabular}
    }
\end{table}

%Please note, however, that this analysis can only be performed for the case where reannotation has been performed and not directly on the output of SelfClean, as it does not make any prediction of the correct label.

Note, however, that the classification of label issues in the four categories correctable, multi-label, neither, and non-agreement follows the point of view of human re-annotation and confident learning correction, specialized to mutually exclusive classes.
The category of label errors defined in our paper is different, as it implies a discrepancy with the actual generating distribution.
For instance, samples where the correct label is neither the one given in the dataset nor the one proposed by confident learning may be actually off-topic in our categorization.
Non-agreement samples may have a clear label and be hard to annotate or be intrinsically ambiguous [5].
The analysis presented above, although very interesting, should be therefore interpreted with care.

\noindent\rule{8cm}{0.4pt}
\begin{displayquote}
    \textit{R.fiv4.4}: The severity of each data quality is not discussed. For example, which issue is the most serious?
\end{displayquote}

The severity of data quality issues was purposely not discussed as this highly depends on the dataset and task, and the identification of general trends depending on the domain and data type deserves separate investigation.
A first, very partial indication can be obtained by comparing Table 3 on the influence of cleaning with Table 16 on issues found in fully automatic mode, as in the answer to R.fiv4.2.
We see the largest effect for Fitzpatrick17k, which mainly contains significant data leakage, followed by DDI, which is very small and contains a few near-duplicates but also some label errors. 
To clarify this point, we added the following as a second paragraph in section 6 "Influence of dataset cleaning":

"The importance of each data quality issue type depends on the dataset and task, and identifying trends by domain and modality requires further investigation.
For the limited number of cases in Table 3, taking into account Table 16, data leaks caused by near duplicates across splits seem to have the highest impact, followed by label errors.
However, we argue that information on off-topic samples and near duplicates within the same data split is always valuable, even if it only serves the purpose of restoring trust."

\noindent\rule{8cm}{0.4pt}
\begin{displayquote}
    \textit{R.fiv4.5}: The reviewer thinks that image quality should also be considered. For example, the image matches the ground truth label well and is not duplicated. However, it can be partially corrupted, have low resolution, be blurry, or have other issues.
\end{displayquote}

We agree with the reviewer that image quality is also an important element for data cleaning.
However, in this submission, we focused on data quality issues that we have found to be prevalent and difficult to detect with standard computer vision methods.
On the one hand, some image quality issues such as corruption or strong blurring may be identified as off-topic samples, as highlighted in the top section of Table 1 for STL+BLUR, VDR+BLUR, and DDI+BLUR.
On the other hand, public data cleaning packages such as CleanLab already cover many image quality aspects (darkness, brightness, odd aspect ratio, odd size, blur, low information) using ad-hoc rules.
We recognize that integrating these rules in the SelfClean package would make it a more complete tool.

This comment prompted us to add the following sentence at the end of the third paragraph of the introduction:
"There are of course other types of data quality issues, including many that can be detected using ad-hoc rules, such as odd brightness, aspect ratio, resolution, sharpness, and entropy in the case of images."

\noindent\rule{8cm}{0.4pt}
\begin{displayquote}
    \textit{R.fiv4.6}: Missing some important baselines. A recent work [3] proposes a benchmark for advanced label error detection methods. It is necessary to compare the SELFCLEAN with these methods.
\end{displayquote}

Thank you for bringing the AQuA benchmark to our attention. 
Please note that in our submission, we formulate the detection problem as a ranking problem and thus also extensively rely on ranking metrics for evaluation.
This differs from AQuA, which evaluates label error detection as a classification problem.
To evaluate SelfClean on AQuA, we would have to rely on automatic cleaning, which conflicts with our recommendation on the methodologies usage (see section 6 "Recommended use").
Nevertheless, for completeness we are trying to include AUM, CIDER, and SimiFeat in our comparison to ensure all benchmarked label cleaning methods are also represented in our evaluation.
We will provide updates as soon as possible.
In the long term, we will also consider extending AQuA to include ranking comparisons.

\noindent\rule{8cm}{0.4pt}
\begin{displayquote}
    \textit{R.fiv4.7}: Synthetic settings may not reflect the data quality issue in real datasets well. One possible solution is to use the CIFAR10H dataset [4] for experiments, which collects 51 judgments per image on average.
\end{displayquote}

We thank the reviewer for suggesting to include an evaluation of label errors on CIFAR10H, which provides a valuable example of natural contamination.
Results show that SelfClean outperforms its competitors by a clear margin for non-agreement and correctable label errors.

Please note, however, that we already present similar experiments on real label errors alongside synthetic label noise. 
These include ImageNet-1k [2] and Food-101N [3], where human reannotation was gathered for a subset of the data, see section 5.2 and appendix H.2.

\begin{table}[htbp]
    \centering
    % \caption{
    %     Comparison of \textsc{SelfClean} and competitor rankings with metadata from multiple benchmark datasets.
    %     We include the proportion of positive samples, which corresponds to the baseline AP.
    % }
    \resizebox{1.0\linewidth}{!}{%
    \begin{tabular}{l c ll rr}
        \toprule
        \bfseries Label Error Type & 
        \bfseries $\text{Positive Samples (\%)}$ & 
        \bfseries Method &
        \bfseries Rep. &
        \bfseries $\text{AUROC (\%)}$ & 
        \bfseries $\text{AP (\%)}$ \\
        
        \midrule
        \multirow{3}{*}{Correctable} & \multirow{3}{*}{0.5} 
            & CLearning & INet & 57.2 & 0.8 \\
        & 
            & FastDup & INet & 68.9 & 0.9 \\
        & 
            & \textsc{SelfClean} & DINO & \textbf{76.3} & \textbf{1.7} \\
        \midrule
        \multirow{3}{*}{Non-agreement} & \multirow{3}{*}{0.7} 
            & CLearning & INet & 56.3 & 0.9 \\
        & 
            & FastDup & INet & 66.8 & 1.2 \\
        & 
            & \textsc{SelfClean} & DINO & \textbf{72.0} & \textbf{3.2} \\
        \bottomrule
    \end{tabular}
    }
\end{table}

\noindent\rule{8cm}{0.4pt}
\begin{displayquote}
    \textit{R.fiv4.8}: Ethical concerns on the usage of CelebA dataset. Please check whether this dataset can be used for experiments according to the work [5].
\end{displayquote}

We thank the reviewer for helping to prevent unethical usage of CelebA.
The outcome of the ethics review was that there is no problem with the usage of CelebA in our submission.
However, following the suggestion from the ethics we added a statement regarding CelebA, addressing potential ethical concerns:

"The CelebA dataset contains images of public figures, and while it is widely used in research, it is important to consider privacy, consent, and potential biases [4]. 
We have ensured that our usage complies with the dataset's terms and conditions, and we advise caution to avoid perpetuating any biases inherent in the dataset. 
Our work does not involve any manipulation or generation of images that could misrepresent individuals."

\subsubsection{Minor Weaknesses}

\begin{displayquote}
    \textit{R.fiv4.9}: The term 'computer vision datasets' is too broad. This paper seems to focus only on image classification tasks.
\end{displayquote}

We agree with the reviewer that the term 'computer vision datasets' is too broad, and thank them for pointing this out.
On the other hand, off-topic samples and near duplicates are not limited to classification tasks.
We thus have changed it to "image datasets" accordingly.

\noindent\rule{8cm}{0.4pt}
\begin{displayquote}
    \textit{R.fiv4.10}: The format in References is inconsistent. One possible option is the IEEE Reference Style Guide.
\end{displayquote}

We thank the reviewer for pointing out the inconsistencies.
The formatting is fixed by the required style file.
We will check all bibtex entries to ensure appropriate reference format.

\noindent\rule{8cm}{0.4pt}
\begin{displayquote}
    \textit{R.fiv4.11}: Many preprint arXiv papers in References have been accepted and published. Please use their official proceedings.
\end{displayquote}

We thank the reviewer for this comment and will update bibtex entries accordingly.

\noindent\rule{8cm}{0.4pt}
\begin{displayquote}
    \textit{R.fiv4.12}: It would be better to move Section D. Evaluation metrics from the appendix to the main paper.
\end{displayquote}

We agree that moving Section D to the main paper would be better and thus changed the submission accordingly.

\noindent\rule{8cm}{0.4pt}
\begin{displayquote}
    \textit{R.fiv4.13}: It would be better to provide more instructions for running the code. README seems too brief. The reviewer fails to find the SSL training codes and pre-trained weights. Could the authors provide more details about them?
\end{displayquote}

We agree with the reviewer that the README can be improved, and will make this a priority.
Tutorials for running the code have also been developed in the meantime and can be provided upon request.
Due to the anonymization platform's limitations, submodules, such as our pre-training weights, are not integrated into the anonymized repository.
However, they will be part of the open-sourced version of the repositories.
If the reviewer would like to see them during the rebuttal, we will find a way to make them accessible.

\noindent\rule{8cm}{0.4pt}
\begin{displayquote}
    \textit{R.fiv4.14}: Is the human verification tool open-sourced?
\end{displayquote}

At the time of the submission, the human verification tool was not yet open-sourced.
However, has been made available in the meantime.
You can access the anonymized repository at:

\begin{center}
    \url{anonymous.4open.science/r/selfclean_verification_tool-BDD2}.
\end{center}

Please note that, while this is useful for reproducibility, it is not a core contribution of our submission and there are other public tools with similar functions.

\subsubsection{References}
[1] Dunnmon, J., Carneiro, G., \& Ré, C. (2020). Hidden Stratification Causes Clinically Meaningful Failures in Machine Learning for Medical Imaging.
\\ \noindent
[2] Northcutt, C. G., Athalye, A., \& Mueller, J. (2021). Pervasive Label Errors in Test Sets Destabilize Machine Learning Benchmarks.
\\ \noindent
[3] Lee, K., He, X., Zhang, L., \& Yang, L. (2017). CleanNet: Transfer Learning for Scalable Image Classifier Training with Label Noise.
\\ \noindent
[4] Peng, K., Mathur, A., \& Narayanan, A. (2021). Mitigating Dataset Harms Requires Stewardship: Lessons from 1000 Papers.
\\ \noindent
[5] Vasudevan, V., Caine, B., Gontijo Lopes, R., Fridovich-Keil, S., \& Roelofs, R. (2022). When Does Dough Become a Bagel? Analyzing the Remaining Mistakes on ImageNet.

\newpage
\section{2nd Comments (21 Aug 24)}

\subsection{Review tscY}
We thank the reviewer for their patience and would like to discuss the requested extension of the human verification experiment.

\noindent\rule{8cm}{0.4pt}
\begin{displayquote}
    \textit{R.tscY.1}: In section 5, the identified label errors with SelfClean are compared with human annotators. I would be interesting to report the same for the other benchmarked methods.
\end{displayquote}

We extended the validation of the algorithmic rankings with humans to include the two best-performing competing methods for each task.
The validation has been performed for ImageNet, a general image dataset, as the rebuttal timeline is insufficient to collect medical expert annotations.
Furthermore, due to ImageNet's size and the rebuttal's timeline, comparing near duplicates is not feasible, as running pHashing and SSIM each take 28 days to compute more than one billion comparisons.

The table compares the percentage of issues found by humans in the 50 lowest-ranked samples with 50 random samples and in samples 1 through 25 with samples 26 through 50.
We report the percentage of issues in each sample and the corresponding $p$-value of a Mann–Whitney $U$ test, which represents the probability for the ranking to be unrelated to the position of positive samples.

The crowdsourced evaluation produced significantly different sample distributions for SelfClean and competing methods.
To cross-check our results against unintended changes, given the large time gap between the initial evaluation and the current one, we repeated the procedure for SelfClean for the very same samples.

The results show a significantly better correspondence of the SelfClean rankings to crowdsourced annotations compared to competitors.
However, there are relatively high fluctuations in significance scores when the experiment is repeated, hinting at a possible low consistency of crowd workers.

\begin{table}[htbp]
    \centering
    \resizebox{\linewidth}{!}{%
        \begin{tabular}{l  l  ccc  ccc }
            \toprule
            & & \multicolumn{6}{c}{\bfseries Percentage of Human-Confirmed Problems} \\
            \cmidrule(lr){3-8}
            
            \bfseries Data Quality Issue &
            \bfseries Method &
            Lowest 1-50 (\%) & Random Sample (\%) & $p$-value &
            Lowest 1-25 (\%) & Lowest 26-50 (\%) & $p$-value \\
            \midrule
            \multirow{4}{*}{Off-topic Samples} &
                HBOS &
                $2$ & $4$ & $0.72$ &
                $0$ & $4$ & $0.84$ \\
            &
                ECOD &
                $2$ & $6$ & $0.85$ &
                $4$ & $0$ & $0.16$ \\
            &
                \textsc{SelfClean} &
                $62 $ & $48 $ & $0.08$ &
                $56 $ & $68 $ & $0.80$ \\
            &
                \textsc{SelfClean} (relabeled) &
                $32$ & $6$ & $\mathbf{4.8 \!\times\!10^{-4}}$ &
                $44$ & $20$ & $\mathbf{0.04}$ \\
            \midrule
            \multirow{4}{*}{Label Errors} &
                FastDup &
                $0$ & $6$ & $0.96$ &
                $0$ & $0$ & $\texttt{undef}$ \\
            & 
                CLearning &
                $4$ & $10$ & $0.88$ &
                $4$ & $4$ & $0.5$ \\
            &
                \textsc{SelfClean} &
                $36 $ & $0 $ & $\mathbf{1.6\!\times\!10^{-6}}$ &
                $48 $ & $24 $ & $\mathbf{0.04}$ \\
            &
                \textsc{SelfClean} (relabeled) &
                $34$ & $14$ & $\mathbf{0.01}$ &
                $44$ & $24$ & $0.07$ \\
            \bottomrule
        \end{tabular}
    }
\end{table}

\newpage
\subsection{Review fiv4}

We thank the reviewer fiv4 for acknowledging our response and raising their score. 

\noindent\rule{8cm}{0.4pt}
\begin{displayquote}
    \textit{R.fiv4.15}: The explanation of the effect of near duplicate samples is not convincing. It would be better for the authors to provide some references (related work) to support the train-evaluation leakage issue.
\end{displayquote}

% - Definition leakage
The cause of data leakage [1, 2] investigated in this submission is the presence of near duplicates across splits [3, 4],
% - Problem with leakage
which results in high performance on the training and evaluation sets but poor generalization to truly unseen data [3].

% - Evidence of prevalence of NDs
In our submission, we conservatively estimate the percentage of errors for 12 image datasets and find that on average 1.8\% of samples are near duplicates of other images.
This is significantly higher than the estimates for off-topic samples (0.1\%) and label errors (0.4\%).
Combined with the fact that some of these datasets, 5 out of 12 of the analyzed ones, do not contain a dedicated train-evaluation split, this results in leakage across splits.

% Impact of NDs on scores
To assess the impact of the data quality issues, we cleaned specific dataset splits in Table 3.
For Fitzpatrick17k, cleaning the evaluation set results in significantly lower performance (-4.1\%pt. in F1).
As 95\% of the data quality issues of Fitzpatrick17k are near duplicates, this effect can be attributed to leakage.
This is a concrete example where the generalization performance is significantly overestimated because of train-evaluation leakage due to near duplicates.

\noindent\rule{8cm}{0.4pt}
\begin{displayquote}
    \textit{R.fiv4.16}: It would be better to compare this work with the AQuA benchmark for completeness. Selecting one or two datasets for comparison would be enough during the rebuttal.
\end{displayquote}

We acknowledge the comment from the reviewer and have accordingly raised the priority of adapting the AQuA benchmark to include an evaluation in terms of ranking performance.
We will post progress updates.

\noindent\rule{8cm}{0.4pt}
\begin{displayquote}
    \textit{R.fiv4.17}: Since this is the dataset/benchmark track, it is necessary for the authors to provide a detailed tutorial/guidebook for reviewers to check reproducibility.
\end{displayquote}

We agree on the importance of reproducibility.
We therefore extended the README of the evaluation repository with the commands to reproduce all experiments.
\begin{center}
    \url{https://anonymous.4open.science/r/SelfClean-Evaluation-0E0F}
\end{center}

The self-supervised training code is accessible at:
\begin{center}
    \url{https://anonymous.4open.science/r/ssl_library-84F8}
\end{center}

\subsubsection{References}

[1] Lones, M. A. (2021). How to avoid machine learning pitfalls: A guide for academic researchers.
\\ \noindent
[2] López, J. A., Chen, B., Saaz, M., Sharma, T., \& Varró, D. (2024). On Inter-dataset Code Duplication and Data Leakage in Large Language Models.
\\ \noindent
[3] Kapoor, S., \& Narayanan, A. (2023). Leakage and the reproducibility crisis in machine-learning-based science. 
\\ \noindent
[4] Abhishek, K., Jain, A., \& Hamarneh, G. (2024). Investigating the Quality of DermaMNIST and Fitzpatrick17k Dermatological Image Datasets.

\newpage
\section{3rd Comments (27 Aug 24)}

% ----------------------
\subsection{Review fiv4}

We thank the reviewer fiv4 for their patience while we ran the requested experiment.

\noindent\rule{8cm}{0.4pt}
\begin{displayquote}
    %\textit{R.fiv4.6}: Missing some important baselines. A recent work [3] proposes a benchmark for advanced label error detection methods. It is necessary to compare the SELFCLEAN with these methods.
    
    \textit{R.fiv4.16}: It would be better to compare this work with the AQuA benchmark for completeness. Selecting one or two datasets for comparison would be enough during the rebuttal.
\end{displayquote}

% Adapting the benchmark to include a comparison of label error rankings turned out to be more difficult than anticipated and would require additional work, which, in the interest of time, was not further pursued.
We compared SelfClean to other methods in terms of binary classification performance for label error detection on CIFAR-10 using the $F_1$ score, as per Table 8 of the AQuA paper [1].
To this end, we apply SelfClean in fully automatic mode, even if this only provides an estimate and should not be used without human supervision, as discussed in Section 6 "Recommended use".
The results show that SelfClean's performance is competitive with the other methodologies and achieves the second-best performance for 3 out of 4 noise types and the third-best for one of them.

\begin{table}[htbp]
    \centering
    \resizebox{1.0\linewidth}{!}{%
    \begin{tabular}{ll cccccc}
        \toprule
        \bfseries Label Error Type & 
        \bfseries AUM & 
        \bfseries CINCER &
        \bfseries CLearning &
        \bfseries SimiFeat &
        \bfseries SelfClean \\
        
        \midrule
        Uniform & 84.9 & 81.7 & 18.1 & \textbf{89.8} & 86.1 \\
        Asymmetric & 85.0 & 85.0 & 18.1 & \textbf{89.0} & 85.9 \\
        Class-dependent & 37.0 & \textbf{64.9} & 37.9 & 58.6 & 38.5 \\
        Instance-dependent & 78.5 & 79.3 & 19.0 & \textbf{83.2} & 79.5 \\
        \bottomrule
    \end{tabular}
    }
\end{table}

A comparison of the ranking for candidate label errors in terms of AUROC and AP would be more informative and fit better in the paper.
Unfortunately extracting scores from the methods included in the AQuA benchmark is not straightforward and would require careful validation, which goes beyond what we can achieve during rebuttal.

% We incorporated the comparison of label error rankings for different methods into the AQuA benchmark.
% Unfortunately including CINCER in this setting requires additional work, and in the interest of time this method is not considered here.
% Below, we report scores for CIFAR-10 with a noise rate of 10\%, similar to the first line in Table 8 of the AQuA paper [1], with the important difference that we compare rankings in terms of average precision.
% The results show that SelfClean outperforms competitors across all four noise types in sorting data quality issues first.

% % AP
% \begin{table}[htbp]
%     \centering
%     \resizebox{1.0\linewidth}{!}{%
%     \begin{tabular}{l c ccccc}
%         \toprule
%         \bfseries Label Error Type &
%         \bfseries $\text{Positive Samples (\%)}$ &
%         \bfseries AUM & 
%         \bfseries CLearning &
%         \bfseries SimiFeat &
%         \bfseries SelfClean \\
        
%         \midrule
%         Uniform & 10.2
%             & 6.1 & 10.4 & 10.2 & \textbf{25.9} \\
%         Asymmetric & 10.0
%             & 6.0 & 10.2 & 9.9 & \textbf{19.8} \\
%         Class-dependent & 47.4
%             & 34.4 & 47.5 & 47.4 & \textbf{57.2} \\
%         Instance-dependent & 14.6
%             & 9.2 & 14.2 & 15.1 & \textbf{24.3} \\
%         \bottomrule
%     \end{tabular}
%     }
% \end{table}

% AUROC
% \begin{table}[htbp]
%     \centering
%     \resizebox{1.0\linewidth}{!}{%
%     \begin{tabular}{l c ccccc}
%         \toprule
%         \bfseries Label Error Type &
%         \bfseries $\text{Positive Samples (\%)}$ &
%         \bfseries AUM & 
%         \bfseries CLearning &
%         \bfseries SimiFeat &
%         \bfseries SelfClean \\
        
%         \midrule
%         Uniform & 10.2
%             & 13.9 & 50.6 & 49.9 & 67.8 \\
%         Asymmetric & 10.0
%             & 16.4 & 50.0 & 50.0 & 67.8 \\
%         Class-dependent & 47.4
%             & 17.7 & 50.1 & 50.0 & 60.8 \\
%         Instance-dependent & 14.6
%             & 15.0 & 48.7 & 50.9 & 64.4 \\
%         \bottomrule
%     \end{tabular}
%     }
% \end{table}

% The differences between the comparison in terms of classification and ranking performance show the importance of comparing methods in both settings.
% Some findings from the paper indeed change when methods are compared in terms of ranking performance.
% Methods considered by AQuA were designed for prediction rather than ranking, which can explain the performance differences.
% The above experiment provides complementary information about the inner workings of the methods, suggesting interesting further investigations.

\subsubsection{References}
[1] Goswami, M., Sanil, V., Choudhry, A., Srinivasan, A., Udompanyawit, C., \& Dubrawski, A. (2023). AQuA: A Benchmarking Tool for Label Quality Assessment.

% ----------------------
\newpage
\subsection{Review qYrV}

We thank reviewer qYrV for their patience while we ran the requested experiments.

\noindent\rule{8cm}{0.4pt}
\begin{displayquote}
    \textit{R.qYrV.3}: Comparisons to SOTA: Authors may be encouraged to compare their method to more methods, e.g., Jia et al 2023, Pleiss et al 2020 etc for off-topic samples.
\end{displayquote}

Reviewer \textit{fiv4} suggested incorporating SelfClean into the AQuA benchmark~[1] for label error detection.
By doing so, we also compared its performance against three additional label error detection methods, including AUM.
We refer to our answer \textit{R.fiv4.16} for results and discussion.

\subsubsection{References}

[1] Goswami, M., Sanil, V., Choudhry, A., Srinivasan, A., Udompanyawit, C., \& Dubrawski, A. (2023). AQuA: A Benchmarking Tool for Label Quality Assessment.


\newpage
\section{After we've done experiments (30 Aug 24)}

\subsection{Overall Comment}
We are grateful to all reviewers for their attentive analysis and for their comments, which greatly improved the manuscript.

% Strengths

% (qYrV)
%- rigorous and innovative approach (-)
%- applicable across various domains
%- methodology is of broad interest to researchers and practitioners (-)
%- methodology well-researched and grounded
%- unique contribution to the field (-)
%- formulation of data cleaning as ranking is innovative
%- SSL strong choice
%- comprehensive experiments/evaluation (-)
%- paper is methodologically sound
%- addressing data quality issues is crucial (-)
%- SelfClean has the potential to improve the reliability of AI
%- well-structured  (-)
%- logical flow
%- transparency and reproducibility

% (tscY)
%- easy to follow (-)
%- proposed method plausible (-)
%- outperforms the SOTA
%- experiments and ablation study are plausible and support claims (-)

% (fiv4)
%- data cleaning highly relevant research topic (-)
%- paper aligns well with the scope of the track (-)
%- proposed method has great potential to help create and maintain image classification datasets
%- experimental results are extensive (-)
%- experiments utilize wide variety of datasets (-)
%- good originality and significance (-)

We are encouraged that they recognize data cleaning to be a crucial (qYrV) and \textbf{highly relevant research topic} (fiv4), which \textbf{aligns well with the track's scope} (fiv4).
It gives us confidence that our analysis is deemed rigorous and innovative (qYrV), plausible (tscY), \textbf{original and significant} (fiv4), and of broad interest to researchers and practitioners (qYrV).
Reviewers also acknowledge that the submission contains a \textbf{comprehensive amount of experiments} and ablation studies (qYrV, fiv4) across a wide variety of datasets (fiv4) and consider them \textbf{to support the claims} (tscY).
It is great to see our effort towards transparency and reproducibility recognized (qYrV).
Last but not least, we are very happy that our submission was found to be \textbf{well-structured} (qYrV) and easy to follow (tscY).

% Points addressed
We also appreciate the valuable and constructive critique of our work.
We {\bf carefully considered all points} raised by the reviewers and addressed them during rebuttal by providing details or running additional experiments. 
Specifically, the discussion led to the following improvements:

\begin{itemize}
    \item The human validation of rankings was extended to competing methods.
    \item CIFAR10H was added to the comparison with metadata.
    \item SelfClean was integrated into the AQuA benchmark and compared to additional label error detection methods based on training dynamics.
    \item Label error detection was separately evaluated for four different types of errors. % for ImageNet-1k
    \item Clarifications have been provided for off-topic samples, severity and diversity of data quality issues, and CelebA's usage.
    %\item Revision of the discussion of off-topic samples to incorporate the hidden stratification phenomenon.
    %\item Addition of a second paragraph to section 6 "Influence of dataset cleaning" discussing the severity of the data quality issues.
    %\item Addition of a statement to the third paragraph of the introduction clarifying that there are more data quality issues, which however can be detected with ad-hoc rules.
    %\item Addition of a statement regarding the usage of CelebA, addressing potential ethical concerns.
    \item We extended the repositories' READMEs with commands to run all experiments.
\end{itemize}

We thank all reviewers and the AC for their consideration and remain at their disposal for additional clarifications.

\end{document}
