# Supplementary material for: Intrinsic Self-Supervision for Data Quality Audits
Source: arXiv:2305.17048 source file (2024-10-28)
Supplement: Supplementary file 3 [file unused_appendices.tex]

% \begin{table}[htbp]
%     \centering
%     \caption{
%         Comparison of the \textsc{SelfClean} ranking with metadata from multiple benchmark datasets.
%         For reference, we include the proportion of positive samples, also corresponding to the not-informed baseline performing best in terms of AP.
%         Please consult section \ref{ssec:naturalresults} for guidance on interpretation.
%     }
%     \label{tab:Detailed-Meta}
%     \begin{tabular}{l l 
%         S[table-format=3.2] % ,table-number-alignment=left (would align the numbers left but it looks better without)
%         S[table-format=3.2]
%         S[table-format=3.2]
%         }
%         \toprule
%         \bfseries Dataset &
%         \bfseries Metadata & 
%         \bfseries $\text{Positive Samples (\%)}$ & 
%         \bfseries $\text{AUROC (\%)}$ & 
%         \bfseries $\text{AP (\%)}$ \\
%         \midrule
%         PAD-UFES-20 & Same Lesion & 0.06 & 71.0 & 10.0 \\
%         PAD-UFES-20 & Not Biopsied & 41.60 & 57.0 & 61.3 \\
%         HAM10000 & Same Lesion & 0.01 & 98.8 & 28.4 \\
%         HAM10000 & Not Follow-Up & 63.89 & 90.8 & 86.3 \\
%         ISIC-2019 & Same Lesion & 0.01 & 98.2 & 26.6 \\
%         CheXpert & Same Patient & 0.01 & 70.5 & 7.5 \\
%         \midrule
%         ImageNet-1k\footnotemark[2] & Verified Label Errors & 88.73 & 67.3 & 8.4 \\
%         Food-101N\footnotemark[3] & Verified Label Errors & 18.51 & 79.8 & 47.8 \\
%         CelebA & Same Person & 0.02 & 78.8 & 30.9 \\
%         \bottomrule
%     \end{tabular}
% \end{table}

\subsection{Performance of pre-trained encoder}
\label{app:Pre-trained-Encoder}
Since \textsc{SelfClean} relies on dataset-specific \gls*{ssl} to produce meaningful latent spaces, the learned features can further be used for transfer learning on the same dataset.
In table \ref{tab:Pre-trained-Performance}, we consider \gls*{dino} pre-training, as performed for \textsc{SelfClean}, on different medical and vision benchmarks, i.e.\ DDI, HAM10000, Fitzpatrick17k, Food-101N, and ImageNet-1k.
The features obtained are compared to a random and supervised ImageNet initialized \gls*{vit} tiny in terms of linear performance on the respective classification task of the datasets, i.e.\ binary classification (benign/malignant) for DDI, multi-class classification for HAM10000, Fitzpatrick17k, Food-101N, and ImageNet-1k.
The results show that ImageNet features perform better for the DDI and ImageNet-1k datasets.
This is not unexpected since DDI is relatively small and the representation was obtained specifically for supervised ImageNet classification.
In contrast, for HAM10000, Fitzpatrick17k, and Food-101N, the features produced by \textsc{SelfClean} are lead to improved results.
This indicates a further benefit of using \textsc{SelfClean}, since the features used for cleaning can be recycled for the considered downstream task where they potentially improve performance.

\begin{table}[htbp]
  \centering
  \caption{
    %\textbf{Linear Performance of Pre-trained Features.} 
    Macro-averaged test F1 scores for multiple vision benchmarks, obtained with linear classifiers on top of different pre-trained feature sets.
    Representations are extracted from a \gls*{vit} tiny using random initialization weights as a baseline, transfer learning from supervised ImageNet, and \gls*{dino} \gls*{ssl} pre-training as performed by \textsc{SelfClean}.
    Results are obtained from runs with three different random seeds, of which we report the average performance and standard error.
    }
  \label{tab:Pre-trained-Performance}
  \resizebox{\linewidth}{!}{%
  \begin{tabular}{
    l  
    S[table-format = 2.2(2)] 
    S[table-format = 2.2(2)]
    S[table-format = 2.2(2)]
    S[table-format = 2.2(2)]
    S[table-format = 2.2(2)]
    }
    \toprule
    \bfseries Method 
        & \multicolumn{1}{r}{\bfseries DDI (\%)} 
        & \multicolumn{1}{r}{\bfseries HAM10000 (\%)} 
        & \multicolumn{1}{r}{\bfseries Fitzpatrick17k (\%)}  
        & \multicolumn{1}{r}{\bfseries Food-101N (\%)} 
        & \multicolumn{1}{r}{\bfseries ImageNet-1k (\%)} \\ 
    \midrule
    Random 
        & 52.5 \pm 1.0
        & 21.9 \pm 0.5
        & 28.9 \pm 0.2
        & 5.1 \pm 0.1
        & 0.8 \pm 0.1 \\
    INet 
        & \bfseries 63.6 \pm 1.1
        & 57.5 \pm 0.4
        & 52.3 \pm 0.1
        & 39.1 \pm 0.1
        & \bfseries 49.1 \pm 0.1 \\
    \textsc{SelfClean} 
        & 59.2 \pm 1.9
        & \bfseries 65.2 \pm 0.4
        & \bfseries 53.8 \pm 0.4
        & \bfseries 53.9 \pm 0.2
        & 34.9 \pm 0.1 \\
    \bottomrule
  \end{tabular}
  }
\end{table}

\subsection{Comparison of self-attention}
In this experiment, we qualitatively compare on selected target datasets the last self-attention block of the encoders trained with \gls*{dino} and supervised ImageNet classification.
This experiment illustrates the difference between self-supervised training on the target domain and domain-agnostic pre-training. 
Figure \ref{fig:Attention-Viz} shows the self-attention masks for a random sample from ImageNet, CheXpert, and Fitzpatrick17k. 
A clear difference is visible for the self-attention masks obtained using the two pre-training strategies.
For example, the masks show that encoders pre-trained with self-supervision attend to many more visual features than their supervised pre-trained counterparts, indicating that self-supervised representations contain more holistic information.

\begin{figure}[htbp]
    \centering
    \captionsetup[subfigure]{justification=centering}
    \begin{subfigure}[b]{0.85\textwidth}
        \begin{subfigure}[b]{\textwidth}
            \centering
            \includegraphics[width=\textwidth]{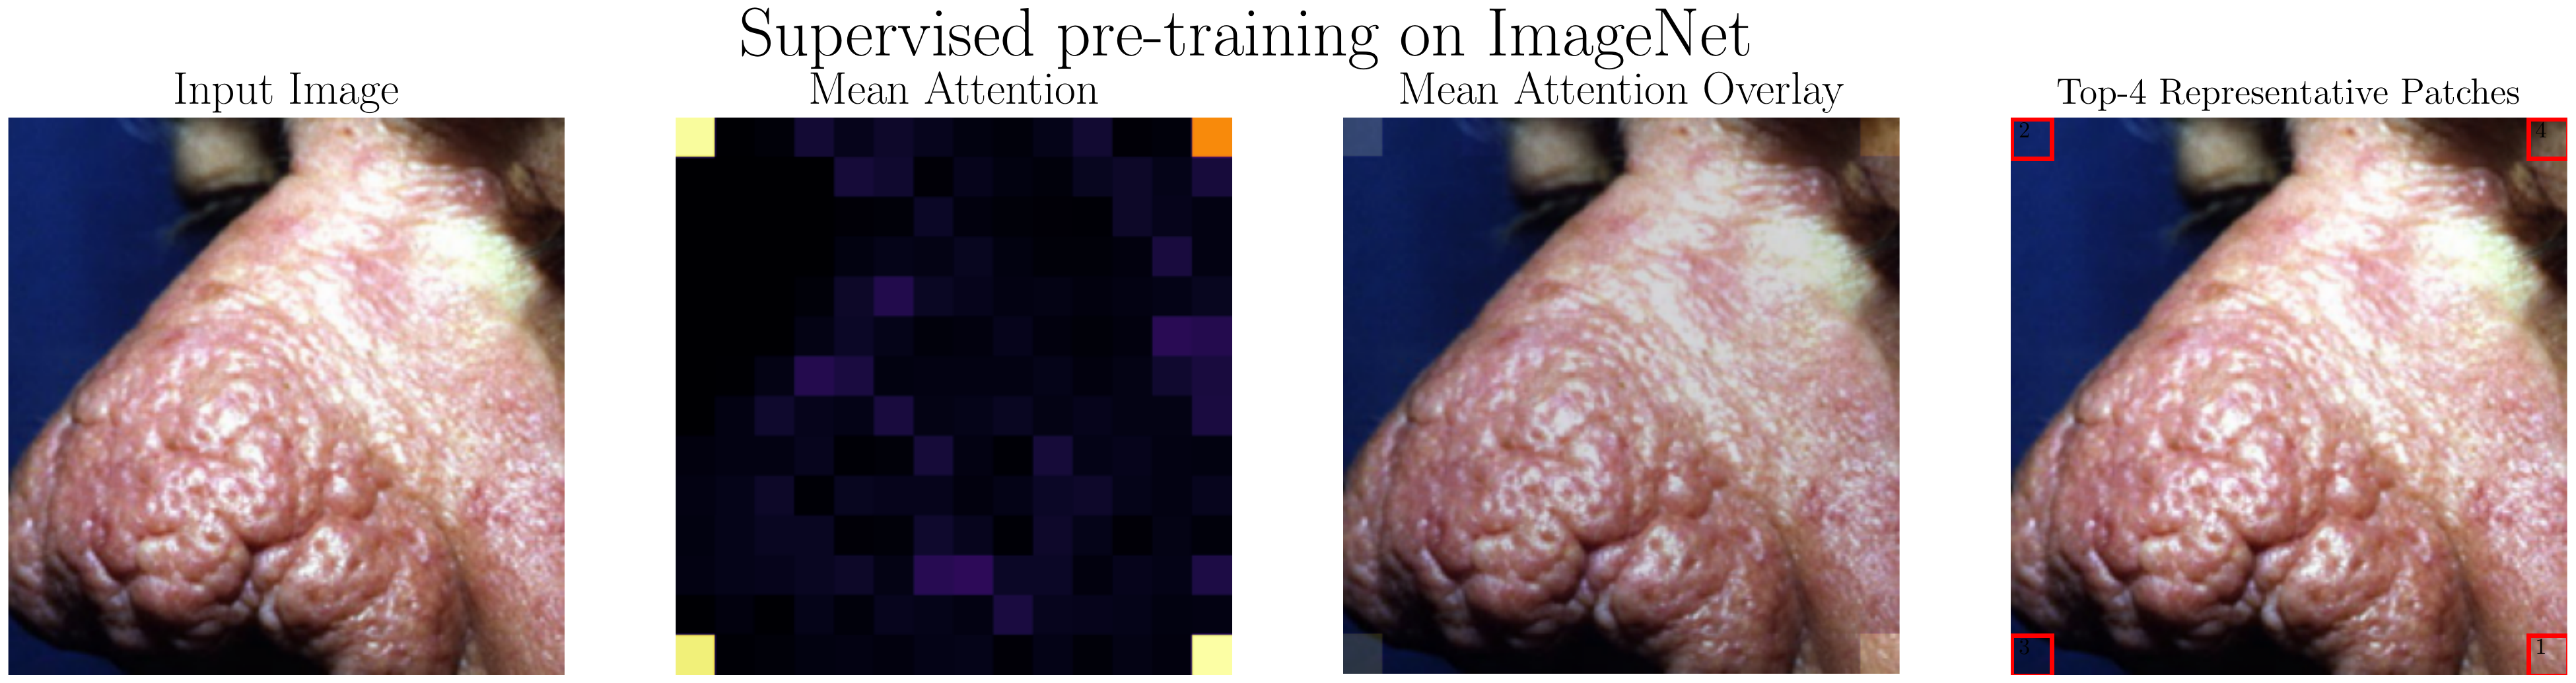}
            %\caption{ImageNet - ViT tiny}
        \end{subfigure}
         
         \begin{subfigure}[b]{\textwidth}
             \centering
             \includegraphics[width=\textwidth]{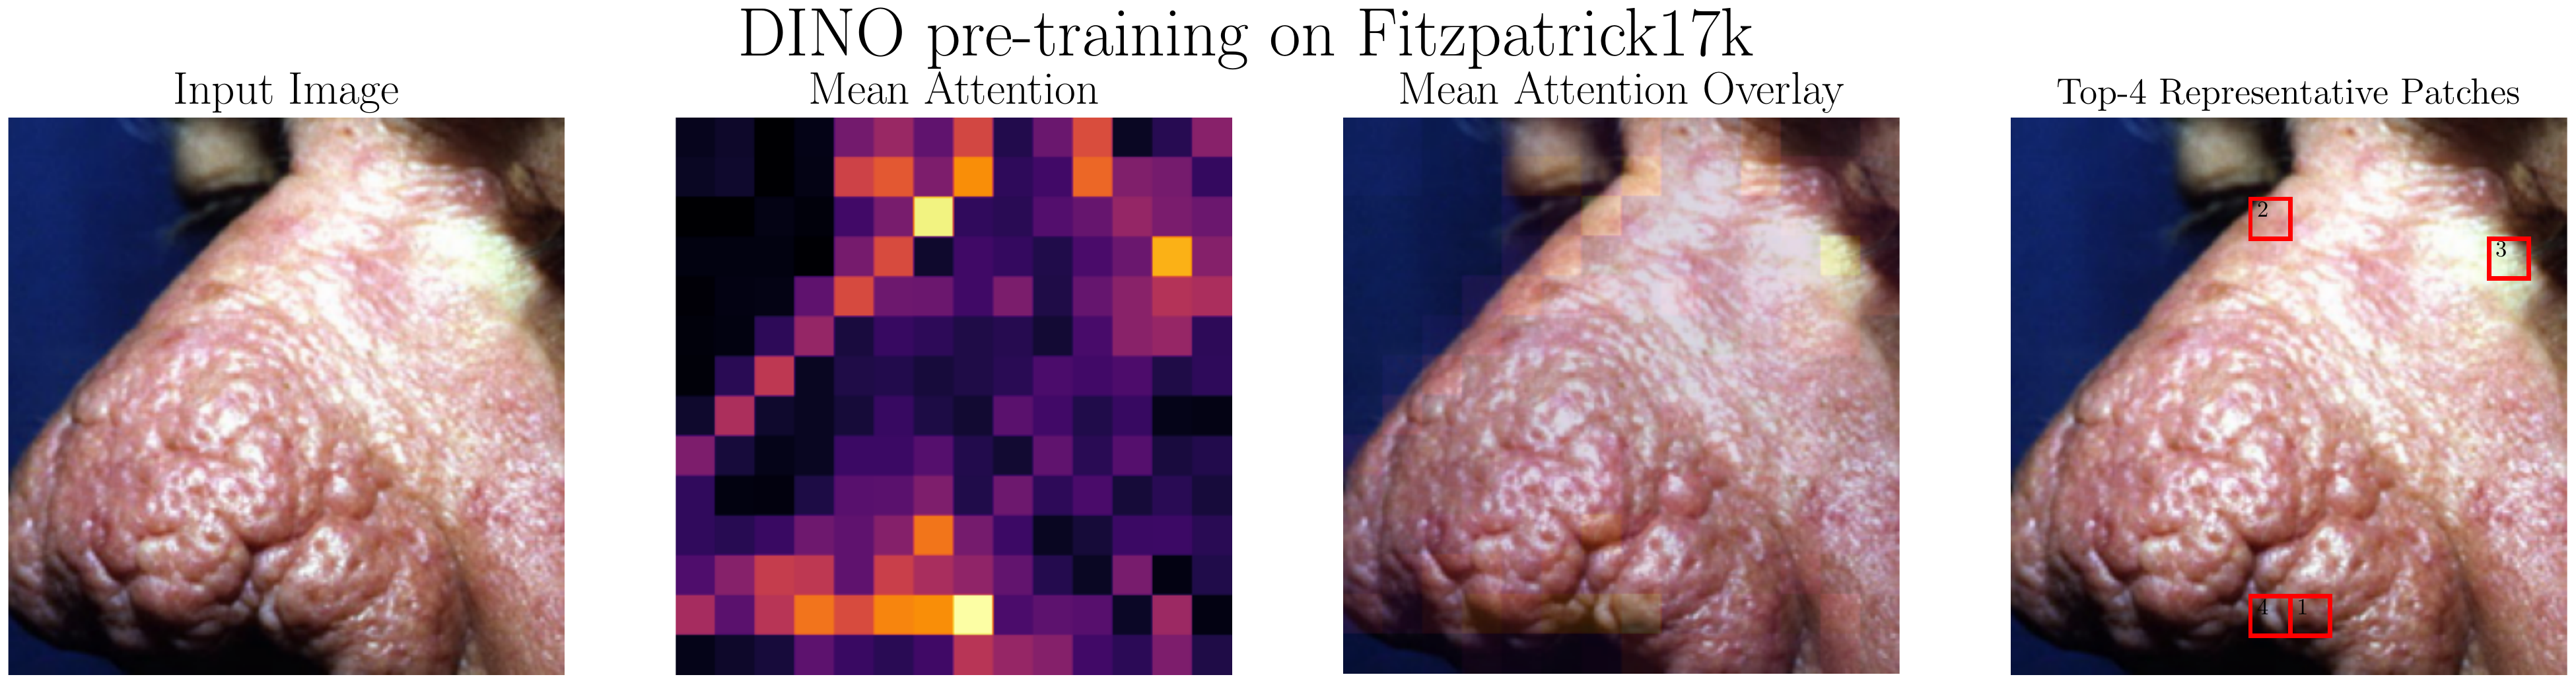}
             %\caption{DINO - ViT tiny}
         \end{subfigure}
         \caption{Fitzpatrick17k \citep{groh_evaluating_2021}}
    \end{subfigure}

    \begin{subfigure}[b]{0.85\textwidth}
        \begin{subfigure}[b]{\textwidth}
            \centering
            \includegraphics[width=\textwidth]{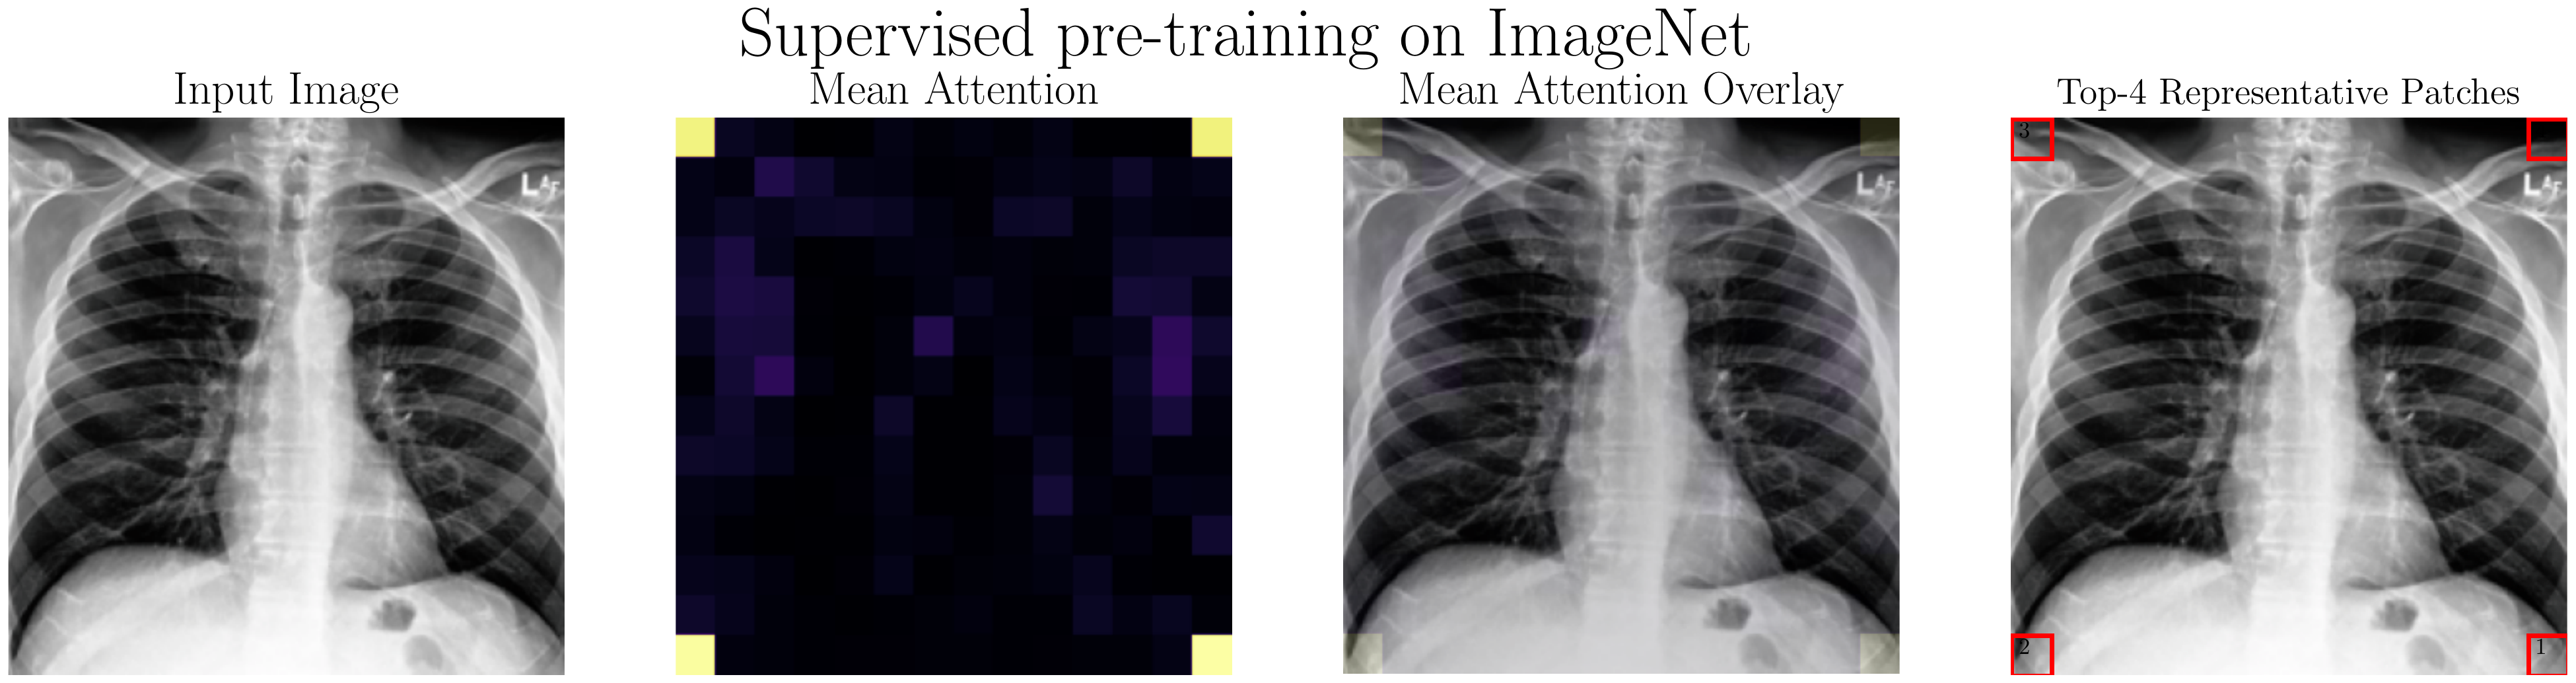}
            %\caption{ImageNet - ViT tiny}
        \end{subfigure}
         
         \begin{subfigure}[b]{\textwidth}
             \centering
             \includegraphics[width=\textwidth]{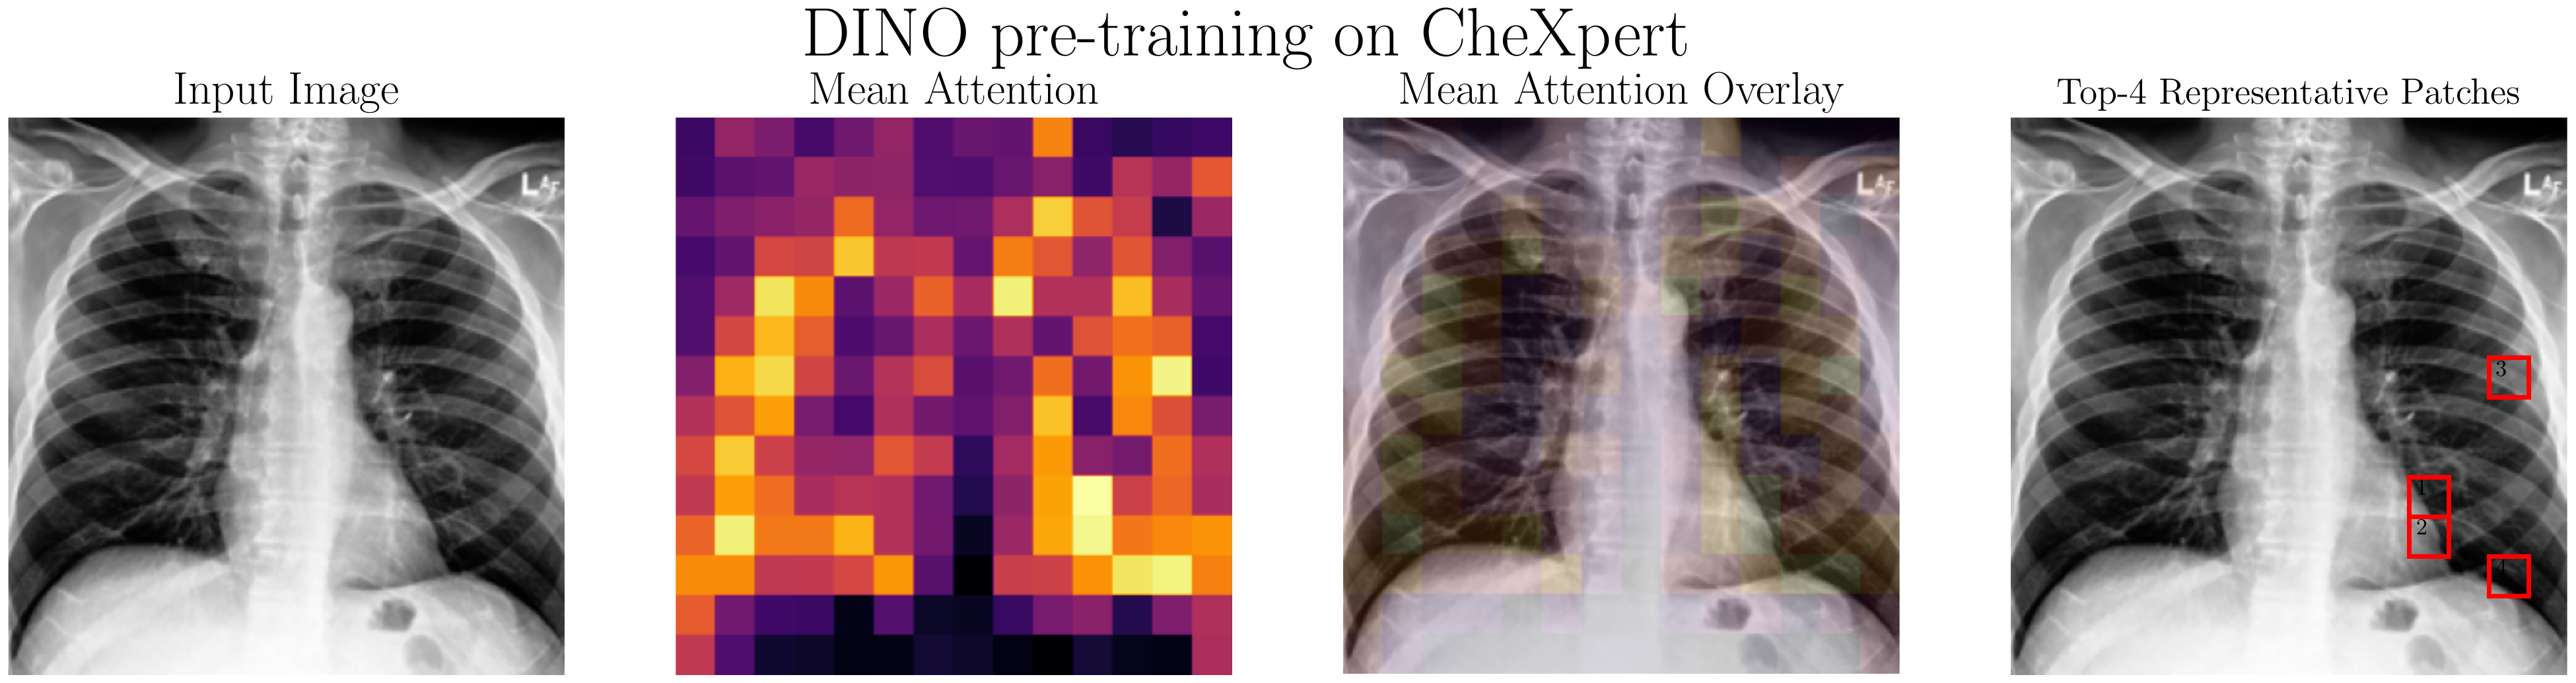}
             %\caption{DINO - ViT tiny}
         \end{subfigure}
    \caption{CheXpert \citep{irvin_chexpert_2019}}
    \end{subfigure}

    \begin{subfigure}[b]{0.85\textwidth}
        \begin{subfigure}[b]{\textwidth}
            \centering
            \includegraphics[width=\textwidth]{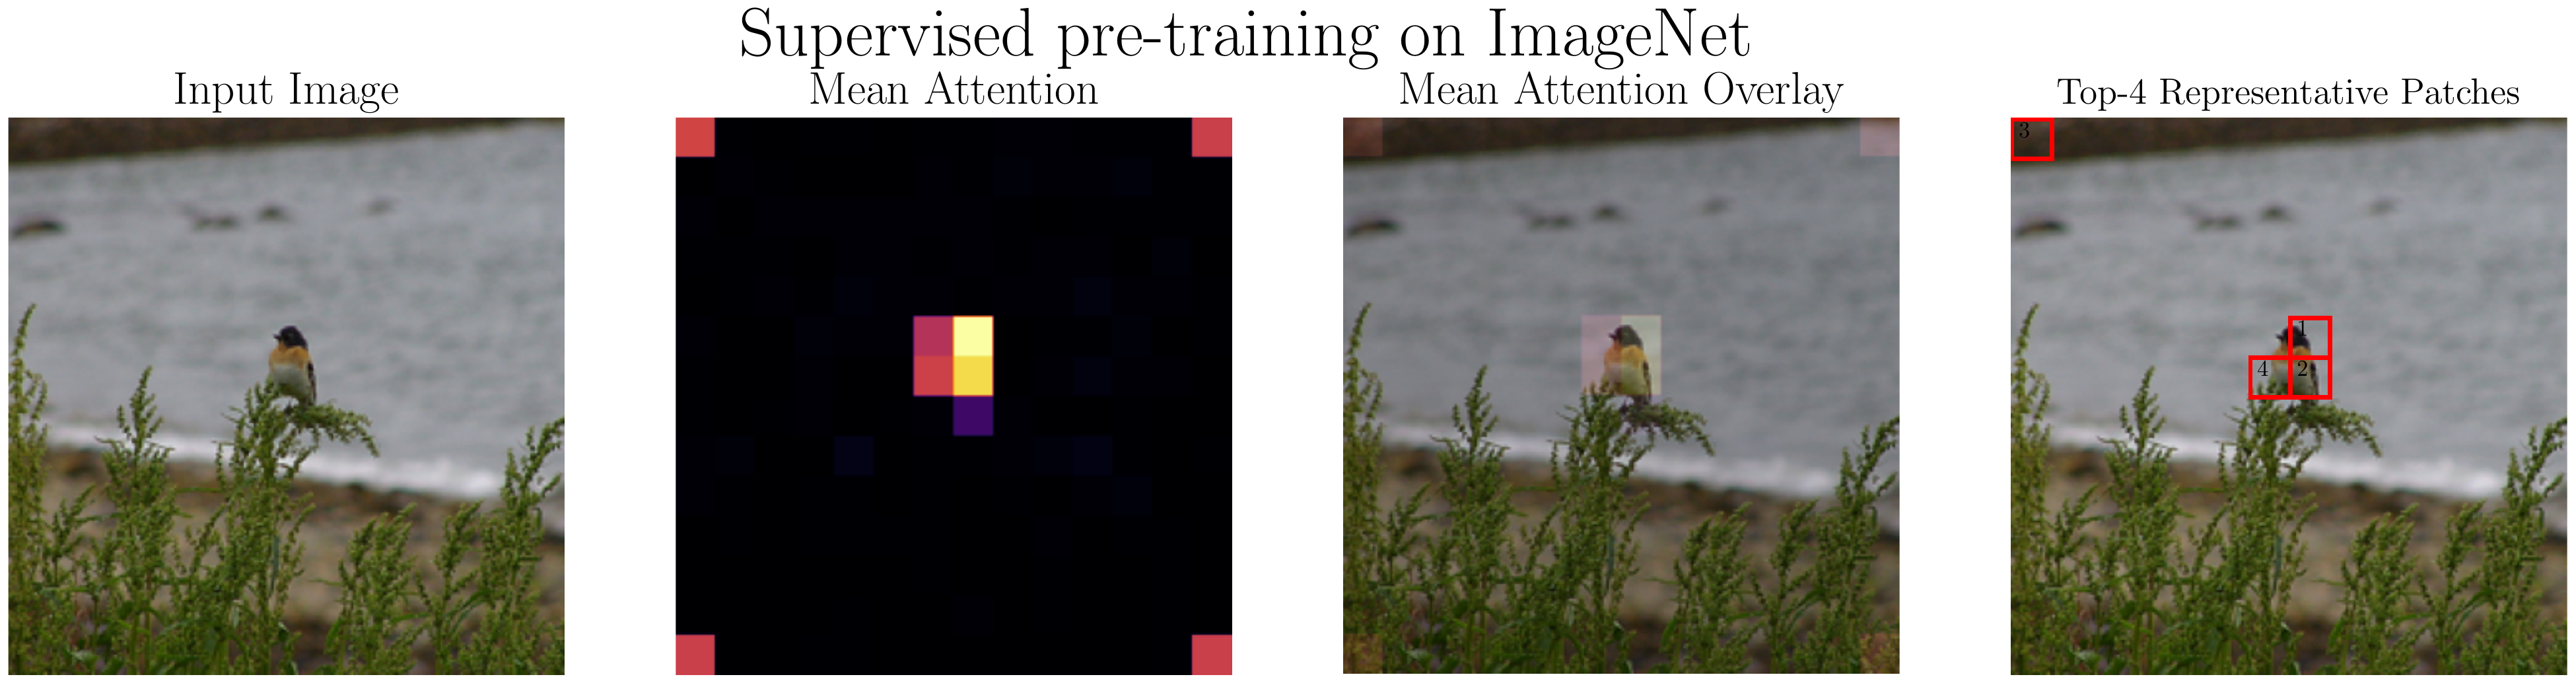}
            %\caption{ImageNet - ViT tiny}
        \end{subfigure}
         
         \begin{subfigure}[b]{\textwidth}
             \centering
             \includegraphics[width=\textwidth]{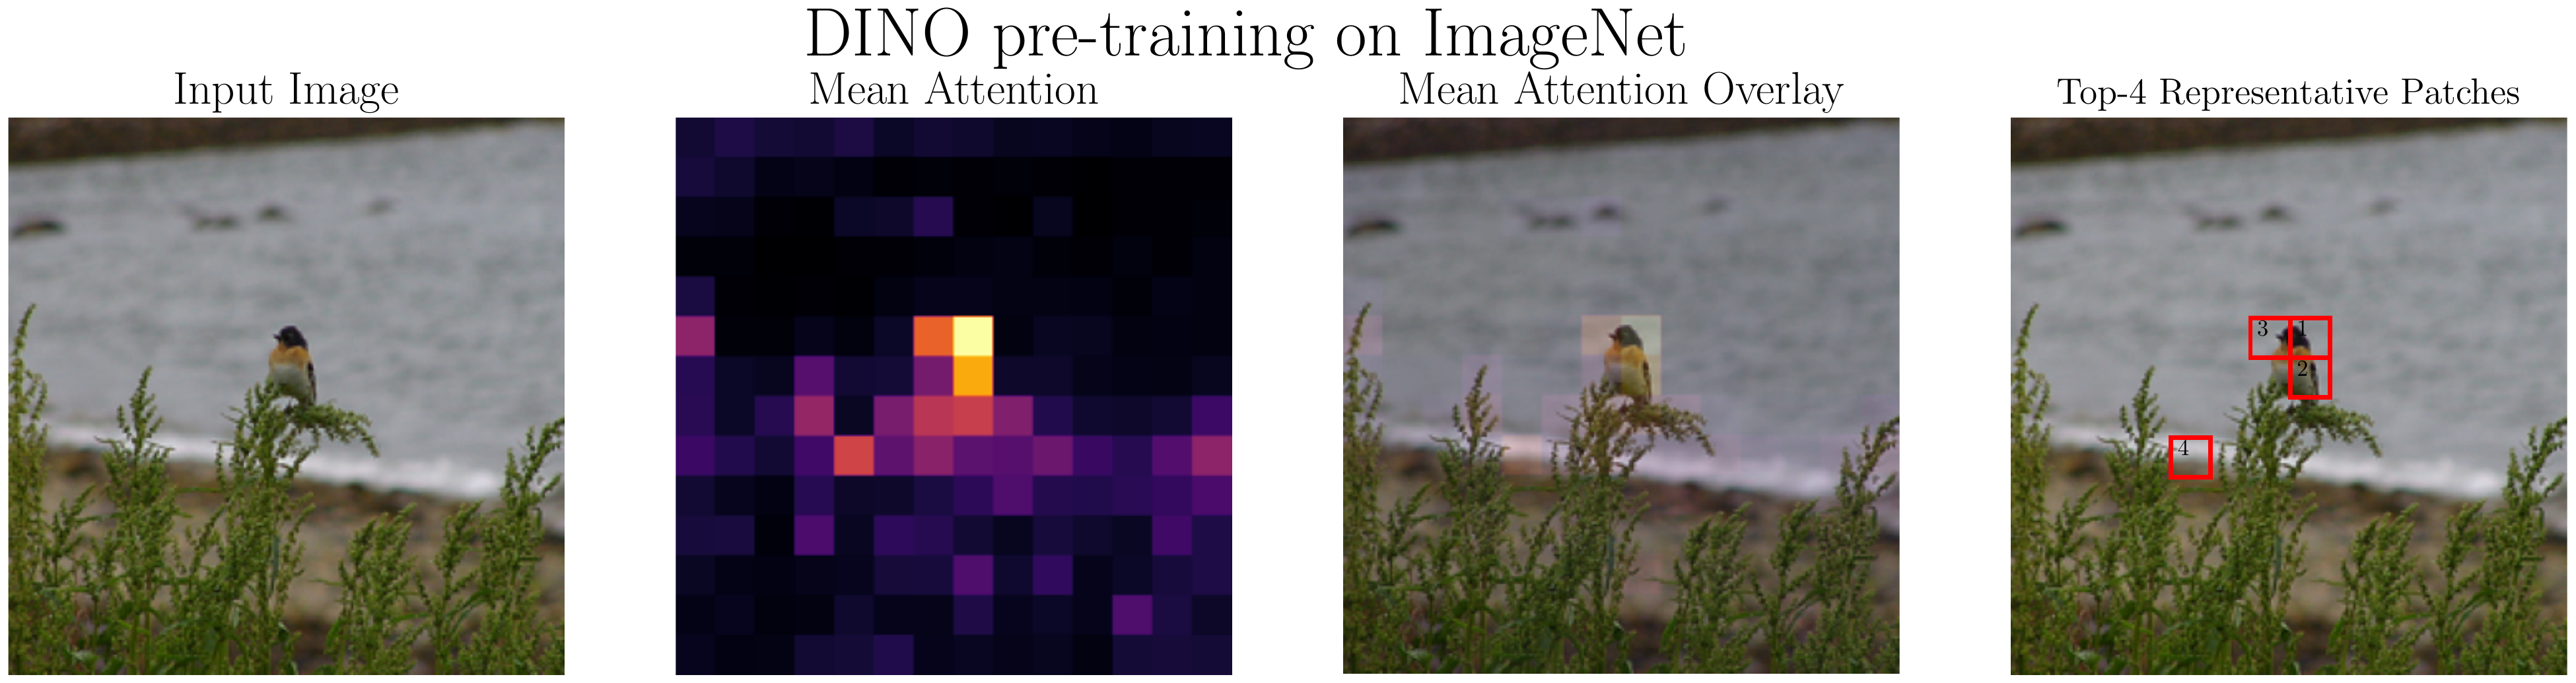}
             %\caption{DINO - ViT tiny}
         \end{subfigure}
         \caption{ImageNet \citep{deng_imagenet_2009}}
    \end{subfigure}
    \caption{
        %\textbf{Self-Attention Visualization.}
        Visualization of the last self-attention block of the encoder pre-trained with supervision on ImageNet and with \gls*{dino} self-supervision on domain-specific datasets, for representative images of different datasets.
        The first column shows the input image, the second the focus of the model computed as the mean self-attention of the last block, the third is an overlay of the first two, and the fourth shows the four most representative patches.
    }
    \label{fig:Attention-Viz}
\end{figure}

\subsection{Investigation of further synthetic augmentations}

The synthetic experiment \protect\ref{app:syntheticcleaningtable} is here repeated with an additional off-topic sample augmentation consisting of strong Gaussian blur with a kernel size of 100 to simulate badly out-of-focus pictures.
This is applied to dataset images at random turning them into off-topic samples, unlike the other synthetic contamination strategies for off-topic samples, i.e. CMED and XR, which add off-topic samples from other sources.

Results show that most baselines fail to detect strongly blurred samples, except for FastDup, which performs well across contaminations and datasets.
This experiment also highlights the benefit of using dataset-specific pre-training as both SimCLR and DINO reach competitive results, whereas the domain-agnostic ImageNet representation achieves significantly lower performance.

\subsection{Mixed Contamination Experiment in Natural Image Domain}

In Figure \ref{fig:MixedContamination-STL-10} we perform the mixed contamination experiment detailed in Section \ref{sec:experimentalsetup} for a natural image dataset, namely STL-10 \citep{coates_analysis_2011}.
Different from experiment \ref{fig:Contamination-Experiment}, we are using synthetic augmentations more closely related to the target domain and thus use BLUR to generate off-topic samples, AUG for near-duplicates, and LBL for label errors.

Results show that \textsc{SelfClean} outperforms the competitive baselines for off-topic samples and near duplicates.
For label errors we can see that FastDup is very competitive and \textsc{SelfClean} with \gls*{dino} is not able to outperform it.
However we can also see that \textsc{SelfClean} with ImageNet features is performing on par with FastDup further highlighting the need for indomain knowledge as ImageNet features are more closely related to STL-10.

\begin{figure}[htbp]
  \includegraphics[width=1.0\linewidth]{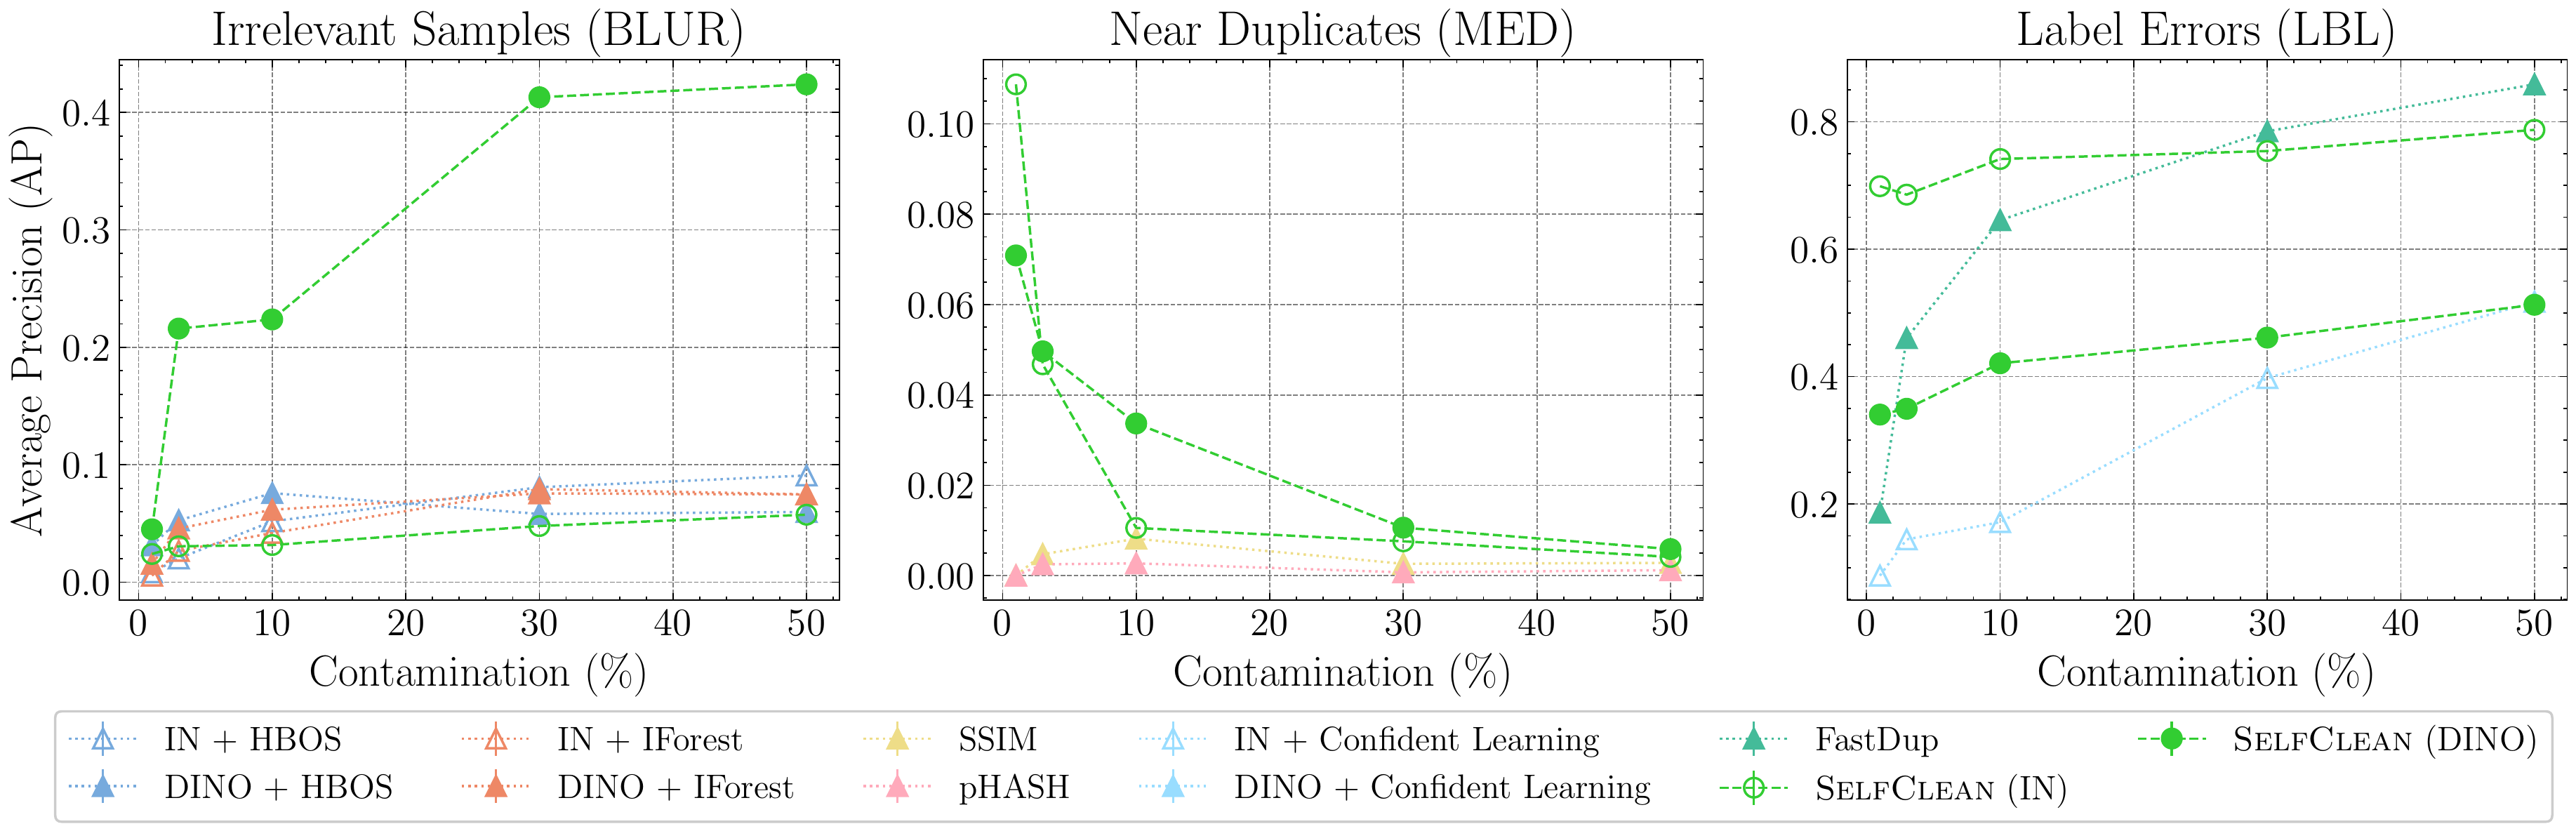}
  \caption{
      Performance of the best two competing approaches for each noise type compared to \textsc{SelfClean} measured on two different representations in terms of AP for a ``mixed-contamination strategy'' when varying the contamination rate.
      The artificial dataset is created from STL-10 by adding strongly blurred images (BLUR), then injecting augmented duplicates (AUG), and finally changing labels at random (LBL).
  }
  \label{fig:MixedContamination-STL-10}
\end{figure}

\section{Fitzpatrick More Visualisations}
\begin{figure}[htbp]
    \begin{subfigure}[b]{0.5\textwidth}
         \centering
         \includegraphics[width=\linewidth]{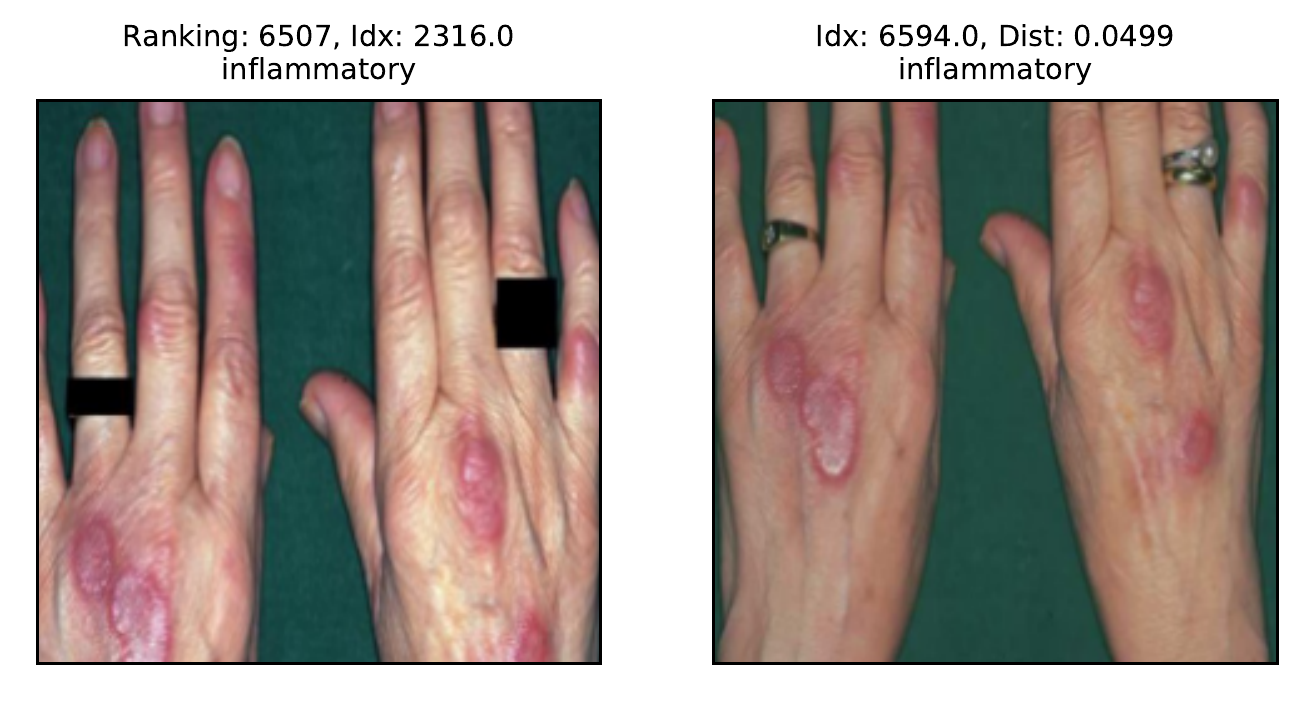}
         \caption{Anonymised Near-Duplicate}
         \label{fig:Dup-Anonym-1}
     \end{subfigure}
     \begin{subfigure}[b]{0.5\textwidth}
        \centering
        \includegraphics[width=\linewidth]{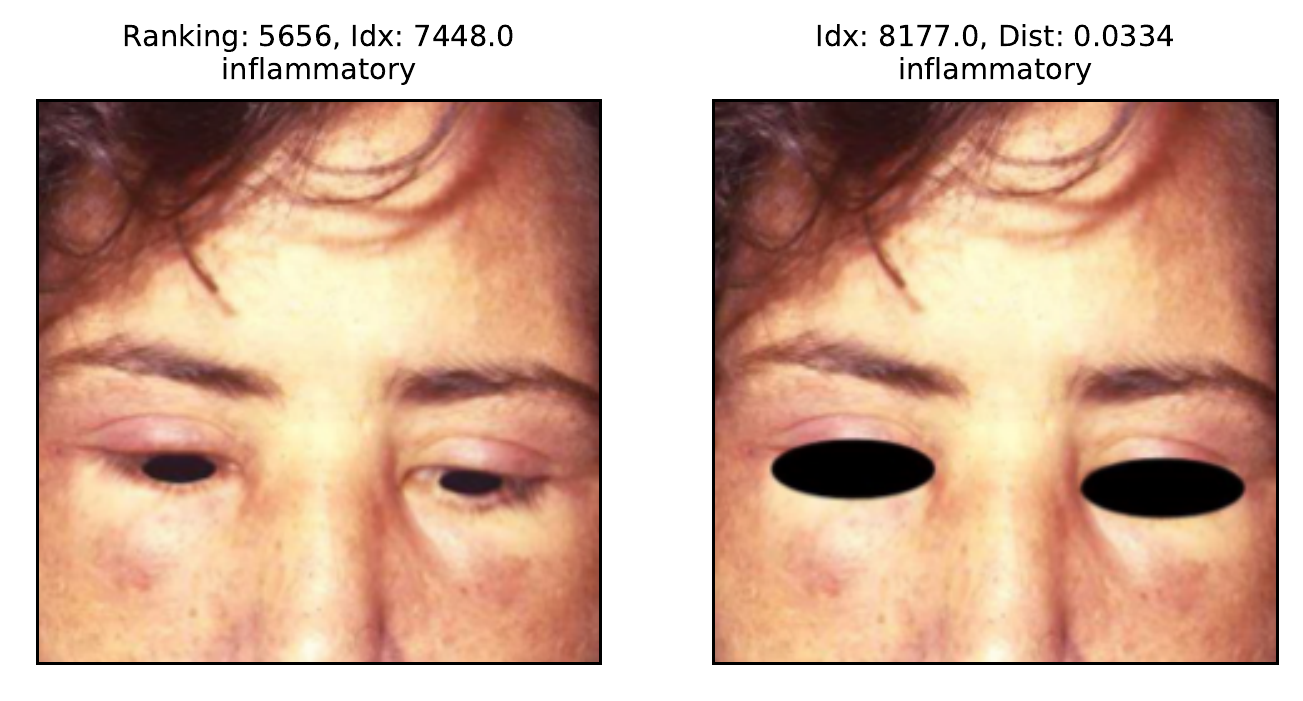}
        \caption{Anonymised Near-Duplicate}
        \label{fig:Dup-Anonym-2}
     \end{subfigure}
     
     \begin{subfigure}[b]{0.5\textwidth}
        \centering
        \includegraphics[width=\linewidth]{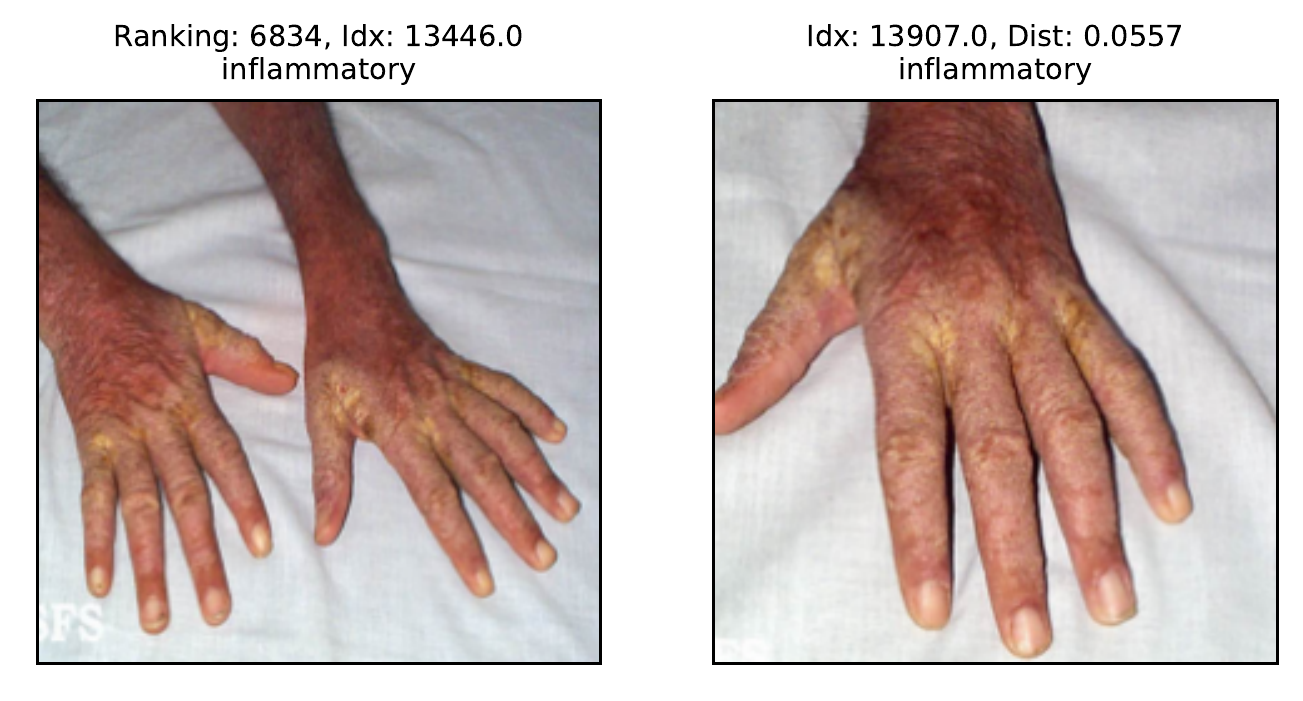}
        \caption{Extreme Near-Duplicate}
        \label{fig:Dup-Extreme-1}
     \end{subfigure}
     \begin{subfigure}[b]{0.5\textwidth}
        \centering
        \includegraphics[width=\linewidth]{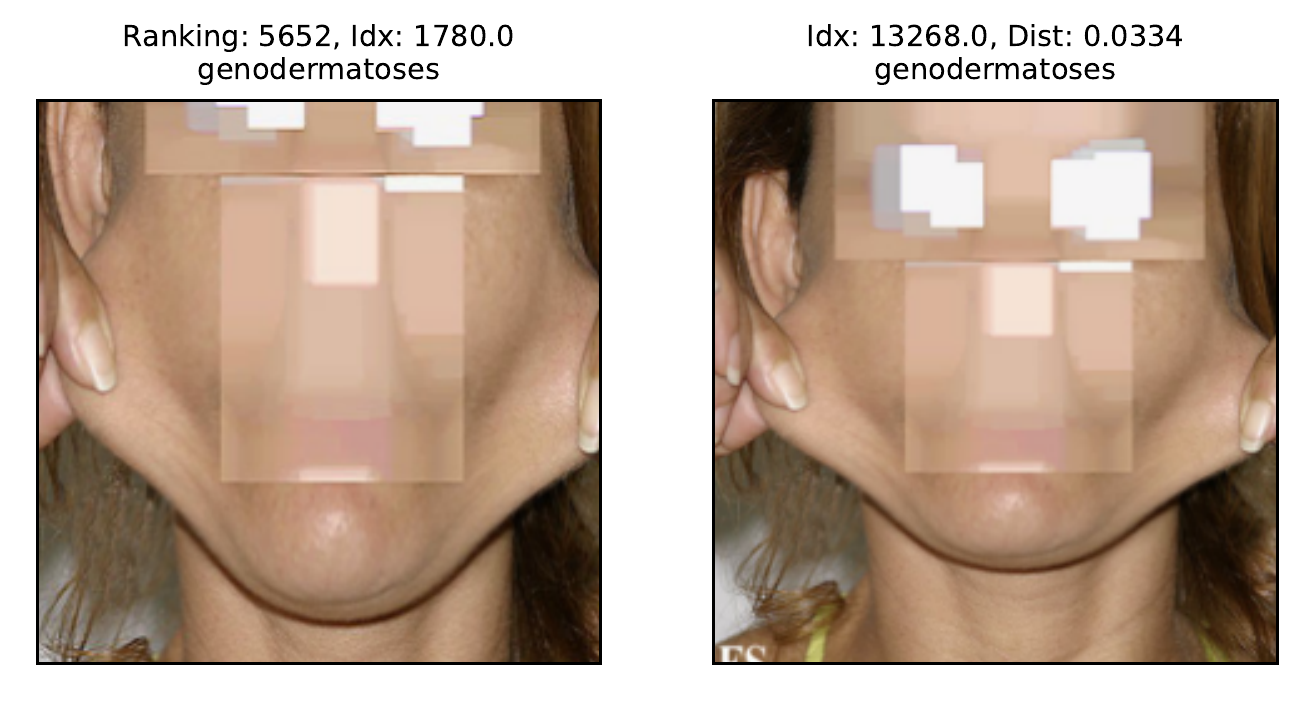}
        \caption{Extreme Near-Duplicate}
        \label{fig:Dup-Extreme-2}
     \end{subfigure}

     \begin{subfigure}[b]{0.5\textwidth}
        \centering
        \includegraphics[width=\linewidth]{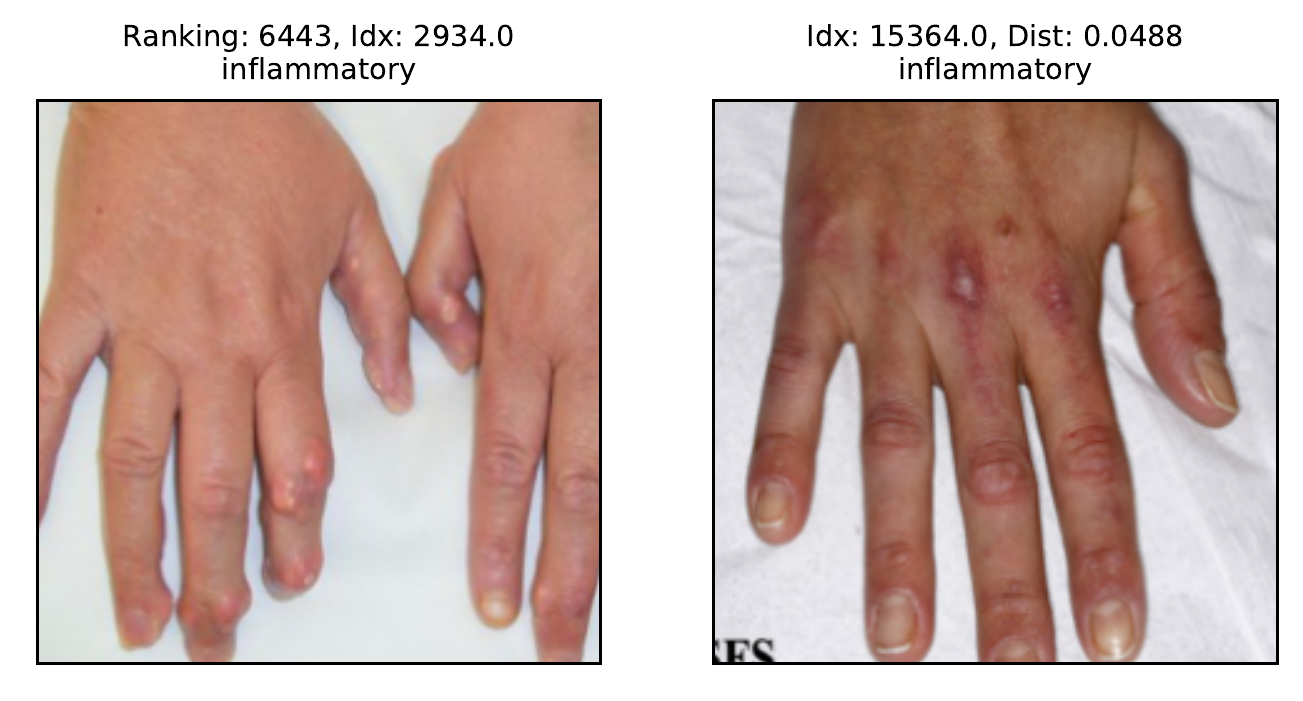}
        \caption{Wrong Near-Duplicate}
        \label{fig:Dup-False-1}
     \end{subfigure}
     \begin{subfigure}[b]{0.5\textwidth}
        \centering
        \includegraphics[width=\linewidth]{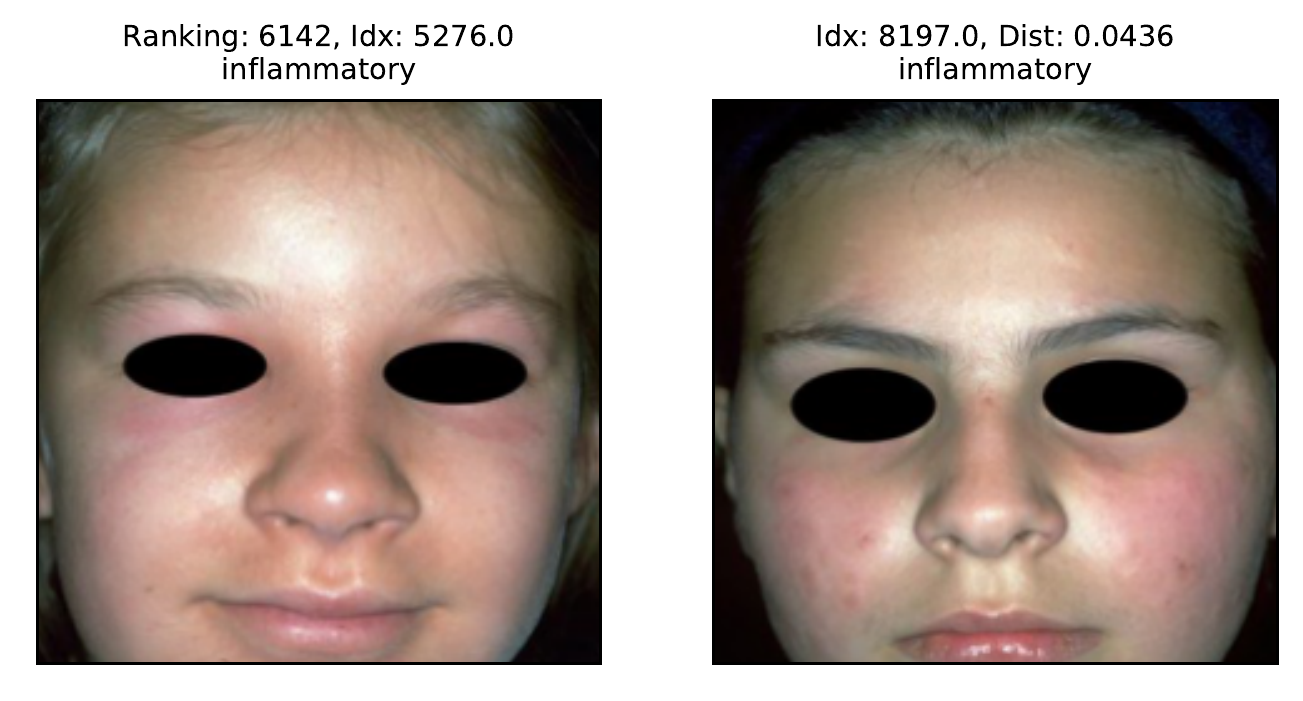}
        \caption{Wrong Near-Duplicate}
        \label{fig:Dup-False-2}
     \end{subfigure}

  \caption{
    %\textbf{Visualization of multiple Fitzpatrick17k near-duplicates.} 
    The figure shows multiple near-duplicates found in the Fitzpatrick17k dataset \citep{groh_evaluating_2021}.
    Figures \ref{fig:Dup-Anonym-1} and \ref{fig:Dup-Anonym-2} show that \textsc{SelfClean} can find near-duplicates where the images were anonymized. 
    Further, figures \ref{fig:Dup-Extreme-1} and \ref{fig:Dup-Extreme-2} show extreme cases of near-duplicates where the method found crops of the same image. 
    Finally, figures \ref{fig:Dup-False-1} and \ref{fig:Dup-False-2} show examples where the near-duplicate detection failed.
}
\label{fig:Gallery-Fitz-Dups}
\end{figure}
